# Supplementary material for: Domain-Agnostic Scalable AI Safety Ensuring Framework
Source: arXiv:2504.20924 source file (2025-10-05)
Supplement: Supplementary file 1 [file supplementary_theory.pdf]

# Domain-agnostic AI Safety-Ensuring Framework - Supplementary Material 1: Theory

## Abstract

This document provides theoretical background, construction, and proof of our research, "Domain-agnostic AI Safety-Ensuring Framework". In section 1 and 2, we explain the structure of our framework. Main theoretical construction regarding safety guarantee is provided in section 3 with our main theorem, Corollary 2. Section 4 and 5 deal with how we can construct loss function and gradient to train the AI model.

## 1 A General Controllable Predict+Optimize Framework

This section deals with the decision-making problem with perception considering user-given parameters. These parameters can be regarded as *knob* for users and used for customizing. Since these parameters are a part of the optimization problem, which is more directly interpretable than an AI model, this method can offer intuitive customization of AI. Moreover, our framework is a *general* form of an optimization problem, including continuous and discrete variables, prediction results of AI model (perception module output), and user-given customization parameters.

This section contains the following: First, we present our general problem setup. Second, we formulate our general framework in which user-given customization parameters are included in the optimization problem. Third, to enable training with this framework, we propose an approximate loss function applicable to general functions using ideas in the ? study, which devised a method to approximate the loss function as a continuous function when the objective is linear. Fourth, we deal with the mathematical calculation of the gradient of the approximate loss function for training and its complexity. Fifth, for the efficiency of the learning process, methods of speeding up optimization, such as warm start and approximation network for integer programming, are introduced.

## 1.1 Problem setup

We want to minimize  $J(\mathbf{u}; \mathbf{s}, \mathbf{r})$  with variable  $\mathbf{u} \in \mathcal{U} \subset \mathbb{R}^{n_{u1}} \times \mathbb{Z}^{n_{u2}}$ , which correspond to the action of our system, under user-given parameters  $\mathbf{r} \in \mathbb{R}^{n_r}$  and environment state  $\mathbf{s} \in \mathcal{S} \subset \mathbb{R}^{n_{s1}} \times \mathbb{Z}^{n_{s2}}$ . Note that bold notations denote vectors. The real objective  $J$  can be unknown, and we cannot directly handle it even if it is known because it is a function of the environment state that we do not have full information about. We can measure  $\mathbf{y}$  that follows the function  $Samp(\mathbf{s})$ , which is the probability distribution of measurement from the environment state, and use it to obtain information about the environment state  $\mathbf{s}$ . Constraints  $c_i(\mathbf{u}; \mathbf{s}, \mathbf{r}) \geq 0$ ,  $i = 1, \dots, n_c$  can also exist. Note that some constraints can depend on the environment state  $\mathbf{s}$  and others do not. Without loss of generality, we assume that  $c_i$  for  $i = 1, \dots, n_{cg}$  do not depend on  $\mathbf{s}$  and  $c_i$  for  $i = n_{cg} + 1, \dots, n_c$  depend on  $\mathbf{s}$ .

## 1.2 Predict+Optimize Framework Formulation

Our approach to the problem in section 1.1 consists of two parts, an AI model that processes measurement results and an optimization stage. The AI model takes the measurement result  $\mathbf{y}$  as the input and generate output  $\mathbf{o} \in \mathcal{O}$ . The processing AI model may consider the user-given parameters for customization  $\mathbf{r}$  as input to obtain tailored output  $\mathbf{o}$  to achieve the best performance under  $\mathbf{r}$ .

Then, we calculate optimal  $\mathbf{u}$  according to the following optimization problem. In the problem,  $\bar{J}(\mathbf{u}; \mathbf{o}, \mathbf{r})$  is the objective of the optimization stage, which is normally similar to real objective  $J(\mathbf{u}; \mathbf{s}, \mathbf{r})$  provided that the output  $\mathbf{o}$  is well processed. Similarly, we have constraints of the optimization stage  $\bar{c}_i(\mathbf{u}; \mathbf{o}, \mathbf{r}) \geq 0$ ,  $i = 1, \dots, n_{\bar{c}}$ , which may partially or fully reflect the real constraints  $c_i(\mathbf{u}; \mathbf{s}, \mathbf{r}) \geq 0$ ,  $i = 1, \dots, n_c$ .

$$\min_{\mathbf{u} \in \mathcal{U} \subset \mathbb{R}^{n_{u1}} \times \mathbb{Z}^{n_{u2}}} \bar{J}(\mathbf{u}; \mathbf{o}, \mathbf{r}) \quad (1a)$$

$$\text{subject to} \quad \bar{c}_i(\mathbf{u}; \mathbf{o}, \mathbf{r}) \geq 0, \quad i = 1, \dots, n_{\bar{c}} \quad (1b)$$

Note that the output of the whole system is  $\mathbf{u}$ , and the performance of the entire system depends only on  $\mathbf{u}$  in general. Nevertheless, we deal with a highly general loss function that can include the optimal objective of the optimization stage or the prediction accuracy.

## 2 Dealing Constraints: Chance-Constrained Method

Safety is one of the most severe problems of AI-based decision-making. Pure machine-learning-based algorithms are trained by only minimizing loss functions, and constraint satisfaction cannot be directly forced. Hence, their safety is not completely guaranteed. Studies have been conducted to ensure safety by projecting the results in a safe area

to overcome this. However, they also have the disadvantages of being suboptimal and failing to guarantee the satisfaction of nondeterministic constraints. This is why pure deep learning-based methods cannot be actively used for safety-sensitive problems like autonomous driving of passenger cars.

This section presents the method that adopts chance-constrained optimization into our general formulation to guarantee constraint satisfaction. To ensure that the constraints are satisfied above the given probability, the performance of the deep learning model is evaluated with labeled sample data before the optimization stage. The probability of each actual situation (environment state) for each result of the deep learning model is calculated based on the prior probability of each situation given as the custom parameters and the evaluation result. Reflecting on this, we determine how conservatively we decide our action (control output) in the optimization stage to satisfy the constraint with a probability above a given value. In the learning stage, the loss function is defined and learned based on the performance of these conservative actions to ensure constraint satisfaction.

This section contains the contents described as follows: First, we provide a general discussion about dealing with constraints in decision-making with perception. Second, we formulate our chance-constrained method to guarantee safety in the framework presented in the former section. Third, we present the technique to obtain conservative action and prove under which conditions and how it can be a valid way for training the chance-constrained method with this framework. Fourth, as a toy example, we apply this method to traffic sign recognition and one-dimensional automotive control problems that reflect the traffic sign to demonstrate its validity.

## 2.1 Constraints: How to deal?

In general, we have some constraints that our actions should satisfy. These constraints can be divided into two groups according to whether they are *deterministic*. *Deterministic* constraints do not depend on the environment state ( $\mathbf{s}$  in problem setup in the former section) since we do not need to measure  $\mathbf{s}$  to know the constraint. Constraints in this group are generally easy to deal with because they can be directly considered in the decision-making stage (optimization stage in our formulation). Even though a method that cannot deal with constraints, such as pure machine learning, is used, the satisfaction of constraint in this group can be guaranteed by postprocessing the action, such as the projection to the constraint-satisfying region.

Conversely, some constraints can be *nondeterministic*. These constraints may depend on  $\mathbf{s}$ ; thus, we should obtain the information about the environment state to satisfy the constraint. Note that constraints that include pure randomness, such as random variables following standard normal distribution, are also classified to this group since such pure

randomness can also be a part of  $\mathbf{s}$ . Nondeterministic constraints cannot be considered directly in the decision-making stage. Instead, we can pursue to satisfy them for larger than a given *probability*. The central concept of this section is obtaining the distribution of  $\mathbf{s}$  and taking our action conservatively to guarantee constraint satisfaction for these constraints over the given probability.

## 2.2 Chance-constrained method

In this subsection, we present the chance-constrained method to guarantee the satisfaction of environment state-dependent constraints ( $c_i$  for  $i = n_{cg} + 1, \dots, n_c$ ). We divide the environment state into parts, including information needed in some constraints and the other part. That is,  $\mathbf{s} = (\mathbf{s}_{cr}(\in \mathcal{S}_{cr}), \mathbf{s}_{ncr}(\in \mathcal{S}_{ncr}))$ ,  $c_i$  for  $i = n_{cg} + 1, \dots, n_c$  are only function of  $\mathbf{s}_{cr}$ . Then, the chance-constraint can be described as follows. Note that the total probability of the dissatisfaction of  $i$ -th original constraint is upper-limited as  $r_{t,i}$ . We assume that a  $(n_c - n_{cg})$ -dimensional vector  $(r_{t,n_{cg}+1}, \dots, r_{t,n_c})$  is also included in  $\mathbf{r}$ .

$$\forall i, Pr(c_i(\mathbf{u}; \mathbf{s}_{cr}, \mathbf{r}) < 0) \leq r_{t,i} \quad (2)$$

To clarify and calculate the left hand side, we also divide the AI model output  $\mathbf{o}$  into  $\mathbf{o} = (\mathbf{o}_{cr}(\in \mathcal{O}_{cr}), \mathbf{o}_{ncr}(\in \mathcal{O}_{ncr}))$  such that the former part includes information about  $\mathbf{s}_{cr}$  and the latter part does not. We call the part of AI model regarding safety classification as *safety classification model*. Moreover, the measurement  $\mathbf{y}$  is also divided into  $\mathbf{y} = (\mathbf{y}_{cr}, \mathbf{y}_{ncr})$ . However,  $\mathbf{y}_{cr}$  is defined as the part needed to obtain  $\mathbf{o}_{cr}$ , and  $\mathbf{y}_{ncr}$  is defined as the remaining part. Thus,  $\mathbf{y}_{cr}$  can include more information than  $\mathbf{s}_{cr}$ . In the remaining part of this section, for simplicity, we only deal with the case that both  $\mathcal{S}_{cr}$  and  $\mathcal{O}_{cr}$  are *finite*. This clearly implies that both  $\mathbf{s}_{cr}$  and  $\mathbf{o}_{cr}$  do not have any continuous part. Dealing with infinite sets remains as a future work and the extension will be further explained in conclusion section.

We apply our previous work ? to our framework (presented in the former section) to ensure constraint satisfaction over the given probability. Specifically, we conduct perception (measurement and postprocessing) for not only the given environment state but also internal test cases with which we already know the environment state. Since it make a challenge that internal test cases will not be changed during training, and thus, can lead to overfitting, we will address the problem in section 3. Then, we merge the result of the internal test cases and user-given prior probability for each possible environment state based on the Bayes rule to obtain posterior probability under the perception output of the real environment state (we do not know). Using these results, we solve the chance-constrained optimization problem under the user-given threshold. To avoid confusion, we use superscript  $r$  for the real thing (environment state, measurement, etc. ) and superscript  $t_i$  for  $i$ th (internal) test case. For example,  $\beta^r$  denotes the real environment

state of the control situation, and  $\beta^{t_i}$  denotes the known environment state of  $i$ th test case.

In addition to the measurement of the real environment state, we also measure the part including information about constraints for each test case. Thus, when we denote  $n_t$  as the number of internal test cases, we obtain (3). Note that  $Samp(\mathbf{s})$  denotes the measurement, which can be treated as a sampling from the probability given by the real environment state  $\mathbf{s}$ . Since  $\mathbf{s}_{cr}^{t_i}$  are fixed,  $\mathbf{y}$  still depends only on  $\mathbf{s}^r$ .

$$\mathbf{y} = (\mathbf{y}^r, \mathbf{y}_{cr}^{t_1}, \dots, \mathbf{y}_{cr}^{t_{n_t}}), \mathbf{y}^r \sim Samp(\mathbf{s}^r), \mathbf{y}_{cr}^{t_i} \sim Samp_{cr}(\mathbf{s}_{cr}^{t_i}) \quad (3)$$

Then, we forward all measurement results in parallel into the AI model like equation (4). Note that  $\mathbf{o}_{cr}(\mathbf{y}_{cr}^{t_i}; \mathbf{r})$  denotes the safety classification model, a part of the original AI model that obtains the part of the output that includes the information about  $\mathbf{s}_{cr}$ . Thus, (4) can be interpreted as a large AI model made by merging one original AI model and  $n_t$  safety classification models in parallel.

$$\mathbf{o}((\mathbf{y}^r, \mathbf{y}_{cr}^{t_1}, \dots, \mathbf{y}_{cr}^{t_{n_t}}); \mathbf{r}) := (\mathbf{o}^r, \mathbf{o}_{cr}^{t_1}, \dots, \mathbf{o}_{cr}^{t_{n_t}}) := (\mathbf{o}(\mathbf{y}^r; \mathbf{r}), \mathbf{o}_{cr}(\mathbf{y}_{cr}^{t_1}; \mathbf{r}), \dots, \mathbf{o}_{cr}(\mathbf{y}_{cr}^{t_{n_t}}; \mathbf{r})) \quad (4)$$

As the next step, we estimate the probability for each output  $\mathbf{o}_{cr}$  under each environment state  $\mathbf{s}_{cr}$ . We denote the elements of  $\mathcal{S}_{cr}$  and  $\mathcal{O}_{cr}$  as  $\mathcal{S}_{cr} = \{\bar{\mathbf{s}}_1, \dots, \bar{\mathbf{s}}_{N_e}\}$  and  $\mathcal{O}_{cr} = \{\bar{\mathbf{o}}_1, \dots, \bar{\mathbf{o}}_{N_o}\}$ . We also let  $\mathbf{1}(a, b)$  as a function that outputs 1 if  $a$  is the same as  $b$  and 0 otherwise, the total number of internal test cases for each environment state as  $N_{\mathbf{s}_{cr}=\bar{\mathbf{s}}_i} = \sum_{k=1}^{n_t} \mathbf{1}(\mathbf{s}_{cr}^{t_k}, \bar{\mathbf{s}}_i)$ , and the number of internal test cases for each output and environment state as  $N_{\mathbf{s}_{cr}=\bar{\mathbf{s}}_i, \mathbf{o}_{cr}=\bar{\mathbf{o}}_j} = \sum_{k=1}^{n_t} \mathbf{1}(\mathbf{s}_{cr}^{t_k}, \bar{\mathbf{s}}_i) \mathbf{1}(\mathbf{o}_{cr}^{t_k}, \bar{\mathbf{o}}_j)$ . Then, under the user-given confidence level  $r_\alpha$  given as a part of  $\mathbf{r}$  (in this paper, we share the confidence level for all probability estimation), the lower and upper bound of the probability for each output under each environment state can be estimated based on the sample proportion as equation (5).

$$p(\mathbf{o}_{cr} = \bar{\mathbf{o}}_j | \mathbf{s}_{cr} = \bar{\mathbf{s}}_i) \simeq \frac{N_{\mathbf{s}_{cr}=\bar{\mathbf{s}}_i, \mathbf{o}_{cr}=\bar{\mathbf{o}}_j}}{N_{\mathbf{s}_{cr}=\bar{\mathbf{s}}_i}} \quad (5)$$

We assume that a  $N_e$ -dimensional vector  $(r_{ep,1}, \dots, r_{ep,N_e})$  that satisfies  $0 \leq r_{ep,k} \leq 1$  and  $\sum_i^{N_e} r_{ep,k} = 1$  is included in  $\mathbf{r}$  as prior knowledge about the probability of each possible environment state associated with constraints. By Bayes rule, we can compute the probability of each environment state under the safety classification model output as equation (6).

$$\begin{aligned} p(\mathbf{s}_{cr} = \bar{\mathbf{s}}_i | \mathbf{o}_{cr} = \bar{\mathbf{o}}_j) &= \frac{p(\mathbf{o}_{cr} = \bar{\mathbf{o}}_j | \mathbf{s}_{cr} = \bar{\mathbf{s}}_i) p(\mathbf{s}_{cr} = \bar{\mathbf{s}}_i)}{p(\mathbf{o}_{cr} = \bar{\mathbf{o}}_j)} \\ &= \frac{p(\mathbf{o}_{cr} = \bar{\mathbf{o}}_j | \mathbf{s}_{cr} = \bar{\mathbf{s}}_i) p(\mathbf{s}_{cr} = \bar{\mathbf{s}}_i)}{\sum_{k=1}^{N_e} p(\mathbf{o}_{cr} = \bar{\mathbf{o}}_j | \mathbf{s}_{cr} = \bar{\mathbf{s}}_k) p(\mathbf{s}_{cr} = \bar{\mathbf{s}}_k)} = \frac{p(\mathbf{o}_{cr} = \bar{\mathbf{o}}_j | \mathbf{s}_{cr} = \bar{\mathbf{s}}_i) r_{ep,i}}{\sum_{k=1}^{N_e} p(\mathbf{o}_{cr} = \bar{\mathbf{o}}_j | \mathbf{s}_{cr} = \bar{\mathbf{s}}_k) r_{ep,k}} \end{aligned} \quad (6)$$

Now, we can obtain the left hand side of (2) as (7) to replace an environment state-dependent constraint based in the method used in ?. Since the measurement and processing for the real environment state are done, and the resulting output  $\mathbf{o}^r$  is obtained, we can obtain the post-perception probability of each environment state based on (6) and the test results. We make the sum of probabilities for possible environment states we neglect not bigger than the given threshold for the specific constraints.

$$\sum_{k:c(\mathbf{u};\bar{\mathbf{s}}_k,\mathbf{r})<0} p(\mathbf{s}_{cr} = \bar{\mathbf{s}}_k | \mathbf{o}_{cr} = \mathbf{o}_{cr}^r) \leq r_{t,i} \quad (7)$$

We can modify (7) based on the big-M method ? to solve it with a solver We adopt integer variables  $\{q_i\}$  to identify the neglecting environment states, Then, we can formulate a set of constraints to replace  $i$ -th ( $i = n_{cg} + 1, \dots, n_c$ ) original constraint as follows.

$$c(\mathbf{u}; \bar{\mathbf{s}}_k, \mathbf{r}) + Mq_k \geq 0, \quad k = 1, \dots, N_e \quad (8a)$$

$$\sum_k p(\mathbf{s}_{cr} = \bar{\mathbf{s}}_k | \mathbf{o}_{cr} = \mathbf{o}_{cr}^r) q_k \leq r_{t,i} \quad (8b)$$

As the final part, we construct a replacement of the environment state-dependent constraints  $c_i$  for  $i = n_{cg} + 1, \dots, n_c$  by compressing the chance-constraint formulation (8). Then, the replacement of  $i$ th original constraint ( $n_{cg} + 1 \leq i \leq n_c$ ) can be written as (9). Note that  $M$  is a sufficiently big constant.

$$\bar{c}_i(\mathbf{u}; \mathbf{o}, \mathbf{r}) := \max_{\substack{s_1, \dots, s_{N_e} \in \{0,1\} \\ \sum_k p(\mathbf{s}_{cr} = \bar{\mathbf{s}}_k | \mathbf{o}_{cr} = \mathbf{o}_{cr}^r) s_k \leq r_{t,i}}} \min_k c(\mathbf{u}; \bar{\mathbf{s}}_k, \mathbf{r}) + M s_k \quad (9)$$

Detailed explanation for our chance-constrained formulation (3),(4),(5),(6),(9) can be found in our former paper ?. Concluding the subsection, we mention that this formulation is a case of the general framework present in Section 1.

**Proposition 1.** *When both  $\mathcal{S}_{cr}$  and  $\mathcal{O}_{cr}$  are finite, our the compressed constraint replacement (9) based on modified chance-constrained formulation (2) is included into our general optimization problem (67). In addition, the whole procedure including the post-processing of the concatenated measurement result and calculation process (3),(4),(5),(6) is included in the general framework presented in Section 1. Moreover, replacements of constraints are continuous with respect to the continuous part of  $\mathbf{u}$  and  $\mathbf{o}$  provided that original constraints to be replaced are continuous with respect to the continuous part of  $\mathbf{u}$ .*

*Proof.* At first, since the environment states of internal test cases are given, the whole measurement depends only on the environment state of the real situation and chance. Then, the measurement can be treated as measuring the real environment state. In

equation (4), the measurement processing AI model can be understood as a new large model to process the concatenated vector. Moreover, the last two equations of (5) and equation (6) can be substituted in equation (9). Since we assume that the part of the output corresponding to the constraints is discrete, continuous outputs have no effect of (9) and are stationary with respect to the continuous part of the AI model output. Furthermore, considering that (9) is constructed by maximum and minimum of finite continuous functions with respect to continuous part of  $\mathbf{u}$ , it is continuous with respect to continuous part of  $\mathbf{u}$ .  $\square$

Note that constraints affected by the continuous part of the environment state  $\mathbf{s}$  or related to the continuous part of the AI model output  $\mathbf{o}$  can be dealt with as constraints in the general framework (67). Although constraint satisfaction cannot be guaranteed, the constraints can also be addressed based on the AI model output, and we can expect satisfaction when the measurement and processing AI model are sufficiently good.

### 3 Conservative Testing with Internal Test Cases

In this section, we present our novel method to train our safety classification model without overfitting problem when we adopt internal test cases. Then, we prove its feasibility and validity under a few assumptions. When we train our safety classification model, the model becomes to depend on the internal test cases. This makes the confidence-level-based robustification technique that is only valid under the assumption that the internal test cases are independent of the parameters of the safety classification model is no more valid. To make the training technique valid, that is, theoretically guaranteed to increase the safety classification model performance when the loss sufficiently decreases, we make the chance-constrained optimization in training conservative, and this leads to training loss becoming an upper bound of the loss when we know the real characteristics of our safety classification model  $p(\mathbf{o}_{cr} = \bar{\mathbf{o}}_j | \mathbf{s}_{cr} = \bar{\mathbf{s}}_i)$ . To do so, we adopt a positive real number  $\xi$  as a conservativeness parameter of training to set and guarantee the conservativeness of chance constraints in training than the reality. This parameter has an important role in proving the validity of the training technique.

#### 3.1 Defining real performance

At first, we mathematically define the real performance at first. We start at a general metric space  $\Omega$  endowed with metric  $M : \Omega \times \Omega \rightarrow [0, \infty]$  and  $\sigma$ -algebra  $\Sigma$ . Then, to treat the measurement of the environment state, we define a probability measure  $P : \Sigma \rightarrow [0, 1]$ . Let  $\mathcal{Y}_{cr}$  denotes the set of possible  $\mathbf{y}_{cr}$ . Then, the conditions for defining the real performance of the safety classification model can be summarized as Condition 1.

**Condition 1.** 1. We can implement a metric  $M_{\mathcal{Y}_{cr}}$  in  $\mathcal{Y}_{cr}$ .

2. We can choose a  $\sigma$ -algebra  $\Sigma_{\mathcal{Y}_{cr}}$ .

3. For each  $\mathbf{s}_{cr}$ , according to  $\text{Samp}_{cr}(\mathbf{s}_{cr})$ , a probability measure  $P_{\mathbf{s}_{cr}} : \Sigma_{\mathcal{Y}_{cr}} \rightarrow [0, 1]$  can be defined.

4. The safety classification model classifies the data into finite potential outputs; that is, the postprocessor can be written as a finite partition of  $\mathcal{Y}_{cr}$  denoted as  $Y_{\bar{\mathbf{o}}_1}, \dots, Y_{\bar{\mathbf{o}}_{N_o}}$ . Moreover,  $Y_{\bar{\mathbf{o}}_j} \in \Sigma_{\mathcal{Y}_{cr}}$  for each  $j$ .

Condition 1 is the essential property needed for mathematical analysis and holds in general. Under Condition 1, the real performance of the safety classification model, that is, the real probability of the output  $\bar{\mathbf{o}}_j$  under environment state  $\bar{\mathbf{s}}_i$ , can be defined as follows.

$$p^*(\mathbf{o}_{cr} = \bar{\mathbf{o}}_j | \mathbf{s}_{cr} = \bar{\mathbf{s}}_i) := P_{\bar{\mathbf{s}}_i}(Y_{\bar{\mathbf{o}}_j}) \quad (10)$$

We can also obtain the replacement of constraints based on (10) similar to (8) and (9) as follows. Note that compared to (9),  $\overline{p(\mathbf{s}_{cr} = \bar{\mathbf{s}}_i | \mathbf{o}_{cr} = \bar{\mathbf{o}}_j)}$  is replaced with  $p^*(\mathbf{s}_{cr} = \bar{\mathbf{s}}_i | \mathbf{o}_{cr} = \bar{\mathbf{o}}_j)$ .

$$p^*(\mathbf{s}_{cr} = \bar{\mathbf{s}}_i | \mathbf{o}_{cr} = \bar{\mathbf{o}}_j) := \frac{p^*(\mathbf{o}_{cr} = \bar{\mathbf{o}}_j | \mathbf{s}_{cr} = \bar{\mathbf{s}}_i) r_{ep,i}}{\sum_{k=1}^{N_e} p^*(\mathbf{o}_{cr} = \bar{\mathbf{o}}_j | \mathbf{s}_{cr} = \bar{\mathbf{s}}_k) r_{ep,k}} \quad (11)$$

$$\bar{c}_i^*(\mathbf{u}; \mathbf{o}, \mathbf{r}) := \max_{\substack{s_1, \dots, s_{N_e} \in \{0,1\} \\ \sum_k p^*(\mathbf{s}_{cr} = \bar{\mathbf{s}}_k | \mathbf{o}_{cr} = \mathbf{o}_{cr}^r) s_k \leq r_{t,i}}} \min_k c(\mathbf{u}; \bar{\mathbf{s}}_k, \mathbf{r}) + M s_k \quad (12)$$

In training, we assume that the measurements of the same set of internal test cases do not change, and we reuse the measurement results  $(\mathbf{y}_{cr}^{t_1}, \dots, \mathbf{y}_{cr}^{t_{n_t}})$  after the first measurement. Since  $(\mathbf{y}_{cr}^{t_1}, \dots, \mathbf{y}_{cr}^{t_{n_t}})$  does not depend on the AI model, it is natural to define the condition of good internal test data for training. The following definition is about how well the internal test cases cover the probability distribution on a set.

**Definition 1.** When there is a compact metric space  $\Omega$  endowed with metric  $M : \Omega \times \Omega \rightarrow [0, \infty]$ ,  $\sigma$ -algebra  $\Sigma$  that includes all open balls, and a probability measure  $P : \Sigma \rightarrow [0, 1]$ , we call a finite sequence of elements of  $\Omega$ ,  $(\omega_1, \dots, \omega_{n_s})$ , is  $\zeta$ -informative if and only if the following statement holds for all subset  $X$  of  $\{1, \dots, n_s\}$ .

$$P(\cup_{i \in X} B(\omega_i, \zeta)) \geq \frac{|X|}{n_s} \quad (13)$$

This implies that the margin  $\zeta$  is robust to the selection of the subset of data. Safety classification model with discrete outputs classifies data and this can be considered as the selection of subsets. Thus, this definition provides robustness for any model or parameters.



Now, we introduce a proposition to guarantee that we can achieve  $\zeta$ -informativeness for arbitrary  $\zeta$  by sampling sufficiently many internal test data from the probability distribution.

**Proposition 2.** *If the support of each  $P$  is connected, when we sample dataset  $D$  following  $P$ , then  $Pr\left(\lim_{|D|\rightarrow\infty} \inf(\{\zeta|D : \zeta\text{-informative}\}) = 0\right) = 1$ .*

*Proof.* Without loss of generality, for simplicity, we assume  $Diam(\Omega) = 1$ . For any  $\delta > 0$ ,  $\{B(\omega, \frac{\delta}{8}) | \omega \in \Omega\}$  is an open cover of  $\Omega$ , and thus, the finite subcover  $\{B(\omega_1, \frac{\delta}{8}), \dots, B(\omega_{n_h}, \frac{\delta}{8})\}$  exists. Let  $H_i := \cup_{j=1}^i B(\omega_j, \frac{\delta}{8}) \setminus \cup_{j=1}^{i-1} B(\omega_j, \frac{\delta}{8})$ ; then,  $\{H_i\}$  is a partition of  $\Omega$  whose elements have a diameter of at most  $\frac{\delta}{4}$ . Since we assume that each  $P$  is well-defined on a  $\sigma$ -algebra that includes all open sets, each  $P$  is well-defined for  $H_i$ . Since  $n_h < \infty$ , we can define  $\rho := \min_{i:P(H_i)>0} P(H_i)$ .

Due to the strong law of large numbers,  $Pr\left(\lim_{|D|\rightarrow\infty} \frac{|D \cap H_i|}{|D|} = P(H_i)\right) = 1$ . Moreover,  $Pr\left(\lim_{|D|\rightarrow\infty} \frac{|D|}{|D|} = P(\Omega)\right) = 1$ . Combining them and considering that  $P(H_i) = \frac{P(H_i)}{P(\Omega)}$ , we obtain

$$Pr\left(\lim_{|D|\rightarrow\infty} \frac{|D \cap H_i|}{|D|} = P(H_i)\right) = 1 \quad (14)$$

provided that  $D \neq \phi$ . This means

$$Pr\left(\exists N, |D| > N \rightarrow \frac{|D \cap H_i|}{|D|} - \frac{\rho}{n_h} \leq P(H_i)\right) = 1 \quad (15)$$

provided that  $D \neq \phi$ .

For any nonempty  $X \subset D$ ,

$$\bigcup_{x \in X} B\left(x, \frac{\delta}{4}\right) \supset \bigcup_{x \in X} \bigsqcup_{i:x \in H_i} H_i = \bigsqcup_{i:X \cap H_i \neq \phi} H_i.$$

Moreover, it is clear that

$$\overline{\bigcup_{x \in X} B\left(x, \frac{3\delta}{4}\right)} \supset \bigcup_{x \in X} B\left(x, \frac{\delta}{2}\right) \quad (16)$$

and furthermore

$$\overline{\Omega \setminus \bigcup_{x \in X} B\left(x, \frac{3\delta}{4}\right)} \cap \overline{\bigcup_{x \in X} B\left(x, \frac{\delta}{2}\right)} = \phi. \quad (17)$$

We note that the overline indicates closure. Then,  $\bigcup_{x \in X} B(x, \frac{\delta}{2})$  and  $\overline{\Omega \setminus \bigcup_{x \in X} B(x, \frac{3\delta}{4})}$  are disjoint open sets of  $\Omega$ . By the assumption that the support is connected, at least one of the following statements holds.

$$S_1. \quad P\left(\overline{\bigcup_{x \in X} B\left(x, \frac{3\delta}{4}\right)} \setminus \bigcup_{x \in X} B\left(x, \frac{\delta}{2}\right)\right) > 0 \quad (18)$$

$$S_2. \quad P\left(\bigcup_{x \in X} B\left(x, \frac{\delta}{2}\right)\right) = 0 \quad (19)$$

$$S_3. \quad P\left(\overline{\Omega \setminus \bigcup_{x \in X} B\left(x, \frac{3\delta}{4}\right)}\right) = 0 \quad (20)$$

To show this, assume all  $S_1, S_2, S_3$  don't hold. Then,  $\text{int}\left(\overline{\bigcup_{x \in X} B\left(x, \frac{3\delta}{4}\right)} \setminus \bigcup_{x \in X} B\left(x, \frac{\delta}{2}\right)\right) \not\subset \text{supp}(P)$  thus  $\text{supp}(P) \subset \overline{\Omega \setminus \bigcup_{x \in X} B\left(x, \frac{3\delta}{4}\right)} \cup \overline{\bigcup_{x \in X} B\left(x, \frac{\delta}{2}\right)}$  where  $\text{int}(\cdot)$  is the interior of set and  $\text{supp}(\cdot)$  is the support of measure. Let  $J = \overline{\bigcup_{x \in X} B\left(x, \frac{\delta}{2}\right)} \cap \text{supp}(P)$  and  $K = \overline{\Omega \setminus \bigcup_{x \in X} B\left(x, \frac{3\delta}{4}\right)} \cap \text{supp}(P)$ , then  $J \cap K = \emptyset$ ,  $J \cup K = \text{supp}(P)$  and both are nonempty since measure is nonzero. Since  $\overline{\bigcup_{x \in X} B\left(x, \frac{\delta}{2}\right)}$  and  $\overline{\Omega \setminus \bigcup_{x \in X} B\left(x, \frac{3\delta}{4}\right)}$  are open sets in  $\overline{\Omega \setminus \bigcup_{x \in X} B\left(x, \frac{3\delta}{4}\right)} \cup \overline{\bigcup_{x \in X} B\left(x, \frac{\delta}{2}\right)}$  (because the complements, which is each other, are closed),  $J$  and  $K$  are open sets in  $\text{supp}(P)$  by definition. Thus it contradicts the assumption that  $\text{supp}(P)$  is connected, and at least one of  $S_1, S_2, S_3$  should hold.

Since we assume that  $D$  is sampled according to  $P$ , the probability of  $S_2$  to hold is 0. Thus, we neglect it.  $S_3$  implies

$$\begin{aligned} P\left(\bigcup_{x \in X} B\left(x, \delta\right)\right) &\geq P\left(\overline{\bigcup_{x \in X} B\left(x, \frac{3\delta}{4}\right)}\right) \\ &= 1 - P\left(\Omega \setminus \overline{\bigcup_{x \in X} B\left(x, \frac{3\delta}{4}\right)}\right) \\ &= 1 \end{aligned} \quad (21) \quad (S_3)$$

If  $S_1$  holds, let

$$T = \overline{\bigcup_{x \in X} B\left(x, \frac{3\delta}{4}\right)} \setminus \bigcup_{x \in X} B\left(x, \frac{\delta}{2}\right). \quad (22)$$

$\bigsqcup_{i: H_i \cap T \neq \emptyset} H_i \supset T$  since  $\{H_i | T \cap H_i \neq \emptyset\}$  is a cover of  $T$ , and  $H_i$  are all disjoint. Thus we obtain

$$\begin{aligned} \sum_{i: H_i \cap T \neq \emptyset} P(H_i) &= P\left(\bigsqcup_{i: H_i \cap T \neq \emptyset} H_i\right) \\ &\geq P(T) \\ &> 0 \end{aligned} \quad (23) \quad (S_1)$$

which implies that there exists  $H_k$  that satisfies  $H_k \cap T \neq \emptyset$  and  $P(H_k) > 0$ . Considering that  $\text{Diam}(H_i) \leq \frac{\delta}{4}$ ,  $H_k \cap T \neq \emptyset$  implies  $H_k \cap (\bigcup_{x \in X} B(x, \frac{\delta}{4})) \neq \emptyset$  and  $H_k \subset \bigcup_{x \in X} B(x, \delta)$ .

Thus,

$$\begin{aligned}
& P\left(\bigcup_{x \in X} B(x, \delta)\right) \\
& \geq P(H_k) + P\left(\bigcup_{x \in X} B\left(x, \frac{\delta}{4}\right)\right) \quad (\text{monotonicity \& additivity of probability}) \\
& \geq \rho + P\left(\bigcup_{x \in X} \bigsqcup_{i: x \in H_i} H_i\right) \quad (\text{monotonicity of probability}) \\
& = \rho + P\left(\bigsqcup_{i: X \cap H_i \neq \phi} H_i\right) \quad (\text{set algebra}) \\
& = \rho + \sum_{i: X \cap H_i \neq \phi} P(H_i) \quad (\text{additivity of probability})
\end{aligned} \tag{24}$$

Moreover, we have

$$\sum_{i: X \cap H_i \neq \phi} \frac{|D \cap H_i|}{|D|} \geq \frac{|X|}{|D|} \tag{25}$$

provided that  $D \neq \phi$  since  $\{H_i | X \cap H_i \neq \phi\}$  is a cover of  $X$ .

Thus, by equation (15), (24), and (25), we obtain

$$Pr\left(\exists N, |D| > N \rightarrow P(\cup_{x \in X} B(x, \delta)) \geq \frac{|X|}{|D|}\right) = 1. \tag{26}$$

Considering that the probability of satisfaction of (19) is 0 and the (20) implies (21), we can conclude that

$$Pr\left(\exists N, |D| > N \rightarrow P(\cup_{x \in X} B(x, \delta)) \geq \frac{|X|}{|D|}\right) = 1, \tag{27}$$

holds for any  $X$ , equivalently,

$$Pr(\exists N, |D| > N \rightarrow D : \delta\text{-informative}) = 1. \tag{28}$$

Moreover, by the definition of  $q(D)$ , this implies that

$$Pr(\exists N, |D| > N \rightarrow \inf(\{\zeta | D : \zeta\text{-informative}\}) \leq \delta) = 1. \tag{29}$$

Therefore, considering that  $\delta$  is an arbitrary positive real number, we obtain

$$Pr\left(\lim_{|D| \rightarrow \infty} \inf(\{\zeta | D : \zeta\text{-informative}\}) = 0\right) = 1. \tag{30}$$

□

### 3.2 Conservative Testing

We can use the idea of *conservative testing* since both  $\mathcal{S}_{cr}$  and  $\mathcal{O}_{cr}$  are finite, that is, introducing a penalty term in the continuous intermediate result of the safety classification model right before the discrete output to obtain robust evaluation result. We can let  $\mathbf{o}_{cr} = \mathbf{g}_{cr}(\mathbf{f}_{cr}(\mathbf{y}; \mathbf{w}_{cr}))$ ,  $\mathbf{f}_{cr}(\mathbf{y}; \mathbf{w}_{cr}) \in R^{m_{cr}}$  and  $\mathbf{1}(\mathbf{o}_{cr}^{t_k}, \bar{\mathbf{o}}_j) = \mathbf{1}(\mathbf{g}_{cr}(\mathbf{f}_{cr}(\mathbf{y}; \mathbf{w}_{cr})), \bar{\mathbf{o}}_j)$  when  $\mathbf{f}_{cr}(\mathbf{y}; \mathbf{w}_{cr})^{t_k}$  is  $\mathbf{f}_{cr}(\mathbf{y}; \mathbf{w}_{cr})$  for  $k$ th (internal) test case. Note that the intermediate output of the postprocessing system  $\mathbf{f}_{cr}(\mathbf{y}; \mathbf{w}_{cr})$  is a function of input of the postprocessing system  $\mathbf{y}_{cr}$ . Now, we do not separate  $\mathbf{o}_{cr}$  ( $= \mathbf{f}_{cr}(\mathbf{y}; \mathbf{w}_{cr})$ ) to their elements for simplicity.

To obtain the conservative result of chance-constrained optimization, we also calculate  $\mathbf{1}^{+\xi}(\mathbf{o}_{cr}^{t_k}, \bar{\mathbf{o}}_j) = \max_{\|\omega_{cr} - \mathbf{f}_{cr}(\mathbf{y}; \mathbf{w}_{cr})^{t_k}\| \leq \xi} \mathbf{1}(\mathbf{g}_{cr}(\omega_{cr}), \bar{\mathbf{o}}_j)$ ,  $\mathbf{1}^{-\xi}(\mathbf{o}_{cr}^{t_k}, \bar{\mathbf{o}}_j) = \min_{\|\omega_{cr} - \mathbf{f}_{cr}(\mathbf{y}; \mathbf{w}_{cr})^{t_k}\| \leq \xi} \mathbf{1}(\mathbf{g}_{cr}(\omega_{cr}), \bar{\mathbf{o}}_j)$ . The intuition is checking that all points in  $\xi$ -ball centered on the  $\mathbf{w}_{cr}$  consistently leads or not leads to the output value  $\bar{\mathbf{o}}_j$ . Note that calculating  $\mathbf{1}^{+\xi}(\mathbf{o}_{cr}^{t_k}, \bar{\mathbf{o}}_j)$  and  $\mathbf{1}^{-\xi}(\mathbf{o}_{cr}^{t_k}, \bar{\mathbf{o}}_j)$  is easy since  $\mathbf{f}_{cr}$  is a simple function in general. Then, we also define the upper bound and the lower bound of the number of internal test cases for each output and environment state as  $N_{\mathbf{s}_{cr}=\bar{\mathbf{s}}_i, \mathbf{o}_{cr}=\bar{\mathbf{o}}_j}^{+\xi} = \sum_{k=1}^{n_t} \mathbf{1}(\mathbf{s}_{cr}^{t_k}, \bar{\mathbf{s}}_i) \mathbf{1}^{+\xi}(\mathbf{o}_{cr}^{t_k}, \bar{\mathbf{o}}_j)$  and  $N_{\mathbf{s}_{cr}=\bar{\mathbf{s}}_i, \mathbf{o}_{cr}=\bar{\mathbf{o}}_j}^{-\xi} = \sum_{k=1}^{n_t} \mathbf{1}(\mathbf{s}_{cr}^{t_k}, \bar{\mathbf{s}}_i) \mathbf{1}^{-\xi}(\mathbf{o}_{cr}^{t_k}, \bar{\mathbf{o}}_j)$ .

Using  $N_{\mathbf{s}_{cr}=\bar{\mathbf{s}}_i, \mathbf{o}_{cr}=\bar{\mathbf{o}}_j}^{+\xi}$  and  $N_{\mathbf{s}_{cr}=\bar{\mathbf{s}}_i, \mathbf{o}_{cr}=\bar{\mathbf{o}}_j}^{-\xi}$ , we can obtain the conservative replacement of  $i$ th original constraint like the former subsection as follows.

$$p^{+\xi}(\mathbf{o}_{cr} = \bar{\mathbf{o}}_j | \mathbf{s}_{cr} = \bar{\mathbf{s}}_i) := \frac{N_{\mathbf{s}_{cr}=\bar{\mathbf{s}}_i, \mathbf{o}_{cr}=\bar{\mathbf{o}}_j}^{+\xi}}{N_{\mathbf{s}_{cr}=\bar{\mathbf{s}}_i}}, p^{-\xi}(\mathbf{o}_{cr} = \bar{\mathbf{o}}_j | \mathbf{s}_{cr} = \bar{\mathbf{s}}_i) := \frac{N_{\mathbf{s}_{cr}=\bar{\mathbf{s}}_i, \mathbf{o}_{cr}=\bar{\mathbf{o}}_j}^{-\xi}}{N_{\mathbf{s}_{cr}=\bar{\mathbf{s}}_i}} \quad (31)$$

$$p^\xi(\mathbf{s}_{cr} = \bar{\mathbf{s}}_i | \mathbf{o}_{cr} = \bar{\mathbf{o}}_j) := \frac{p^{+\xi}(\mathbf{o}_{cr} = \bar{\mathbf{o}}_j | \mathbf{s}_{cr} = \bar{\mathbf{s}}_i) r_{ep,i}}{\sum_{k=1}^{N_e} p^{-\xi}(\mathbf{o}_{cr} = \bar{\mathbf{o}}_j | \mathbf{s}_{cr} = \bar{\mathbf{s}}_k) r_{ep,k}} \quad (32)$$

$$\bar{c}_i^\xi(\mathbf{u}; \mathbf{o}, \mathbf{r}) := \max_{\substack{s_1, \dots, s_{N_e} \in \{0,1\} \\ \sum_k p^\xi(\mathbf{s}_{cr}=\bar{\mathbf{s}}_k | \mathbf{o}_{cr}=\mathbf{o}_{cr}^r) s_k \leq r_{t,i}}} \min_k c_i(\mathbf{u}; \bar{\mathbf{s}}_k, \mathbf{r}) + M s_k \quad (33)$$

Note that (33) is replacement of  $c_i(\mathbf{u}; \bar{\mathbf{s}}_k, \mathbf{r})$  (to obtain action based on output  $\mathbf{o}$  rather than environment state  $\mathbf{s}$ , and thus, we use  $c_i(\mathbf{u}; \bar{\mathbf{s}}_k, \mathbf{r})$  in the minimum in (33). Since  $\mathbf{1}^{-\xi}(\mathbf{o}_{cr}^{t_k}, \bar{\mathbf{o}}_j) \leq \mathbf{1}(\mathbf{o}_{cr}^{t_k}, \bar{\mathbf{o}}_j) \leq \mathbf{1}^{+\xi}(\mathbf{o}_{cr}^{t_k}, \bar{\mathbf{o}}_j)$ , It is straightforward that  $p^\xi(\mathbf{s}_{cr} = \bar{\mathbf{s}}_k | \mathbf{o}_{cr} = \mathbf{o}_{cr}^r) \geq p(\mathbf{s}_{cr} = \bar{\mathbf{s}}_k | \mathbf{o}_{cr} = \mathbf{o}_{cr}^r)$  and  $\bar{c}_i^\xi(\mathbf{u}; \mathbf{o}, \mathbf{r}) \leq \bar{c}_i(\mathbf{u}; \mathbf{o}, \mathbf{r})$ .

Then, we can characterize the condition in addition to Condition 1 that guarantees the conservativeness of (33) as follows.

**Condition 2.** For some  $(\zeta, \xi)$ ,

1.  $\Sigma_{\mathcal{Y}_{cr}}$  includes all open balls (based on  $M_{\mathcal{Y}_{cr}}$ ).
2. For each  $\bar{\mathbf{s}}_i$ , subsequence  $(\mathbf{y}_{cr}^{t_{a_1}}, \dots, \mathbf{y}_{cr}^{t_{a_{N^{at}}}}) : \{a_j\} = \{k | \mathbf{s}_{cr}^{t_k} = \bar{\mathbf{s}}_i\}$ , that is subsequence consists of the sampled measurement result of environment state  $\bar{\mathbf{s}}_i$  of the sequence  $(\mathbf{y}_{cr}^{t_1}, \dots, \mathbf{y}_{cr}^{t_{n_t}})$ , is  $\zeta$ -informative in  $(\mathcal{Y}_{cr}, M_{\mathcal{Y}_{cr}}, \Sigma_{\mathcal{Y}_{cr}}, P_{\bar{\mathbf{s}}_i})$ .
3.  $\mathbf{w}_{cr}(\mathbf{y}_{cr})$  satisfies that  $\|\mathbf{w}_{cr}(v_1) - \mathbf{w}_{cr}(v_2)\| \leq \xi$  if  $M_{\mathcal{Y}_{cr}}(v_1, v_2) < \zeta$  for any  $v_1, v_2 \in$

$\mathcal{Y}_{cr}$ .

Condition 2 is about the required quality of the supplementary data and the required property of the safety classification model. With big  $\zeta$ , many sequences are  $\zeta$ -informative. Big  $\xi$  allows many neural networks and large  $\zeta$  to satisfy the condition. However, a large  $\xi$  makes our system much extensively conservative. In contrast, only high-quality samples can be  $\zeta$ -informative for low  $\zeta$ , and the stiffness of the AI model should be low to satisfy the condition with small  $\xi$ . But, small  $\xi$  allows less conservative actions. Now, we can prove the conservativeness of (33), based on the conditions.

**Theorem 1.** *Under Condition 1 and Condition 2,*

$$p^{-\xi}(\mathbf{o}_{cr} = \bar{\mathbf{o}}_j | \mathbf{s}_{cr} = \bar{\mathbf{s}}_i) \leq p^*(\mathbf{o}_{cr} = \bar{\mathbf{o}}_j | \mathbf{s}_{cr} = \bar{\mathbf{s}}_i) \leq p^{+\xi}(\mathbf{o}_{cr} = \bar{\mathbf{o}}_j | \mathbf{s}_{cr} = \bar{\mathbf{s}}_i). \quad (34)$$

*Proof.* For the first inequality, by definition, we obtain

$$p^{-\xi}(\mathbf{o}_{cr} = \bar{\mathbf{o}}_j | \mathbf{s}_{cr} = \bar{\mathbf{s}}_i) = \frac{|\{k | \mathbf{s}_{cr}^{t_k} = \bar{\mathbf{s}}_i, \mathbf{f}_{cr}(\bar{B}(f(\mathbf{y}_{cr}^{t_k}; \mathbf{w}_{cr}), \xi)) = \{\bar{\mathbf{o}}_j\}\}|}{N_{\mathbf{s}_{cr}=\bar{\mathbf{s}}_i}} \quad (35)$$

when  $\bar{B}(\mathbf{y}_{cr}^{t_k}, \xi)$  denotes the closed ball centered on  $\mathbf{y}_{cr}^{t_k}$  with radius  $\xi$ .

Meanwhile, by the third statement of Condition 2,  $f(\bar{B}(f(\mathbf{y}_{cr}^{t_k}; \mathbf{w}_{cr}), \xi)) = \{\bar{\mathbf{o}}_j\}$  implies  $B(\mathbf{y}_{cr}^{t_k}, \zeta) \subset Y_{\bar{\mathbf{o}}_j}$ . By substituting this in (35) and using the second statement of Condition 2, we obtain

$$p^{-\xi}(\mathbf{o}_{cr} = \bar{\mathbf{o}}_j | \mathbf{s}_{cr} = \bar{\mathbf{s}}_i) = \frac{|\{k | \mathbf{s}_{cr}^{t_k} = \bar{\mathbf{s}}_i, f(\bar{B}(f(\mathbf{y}_{cr}^{t_k}; \mathbf{w}_{cr}), \xi)) = \{\bar{\mathbf{o}}_j\}\}|}{N_{\mathbf{s}_{cr}=\bar{\mathbf{s}}_i}} \leq \frac{|\{k | \mathbf{s}_{cr}^{t_k} = \bar{\mathbf{s}}_i, B(\mathbf{y}_{cr}^{t_k}, \zeta) \subset Y_{\bar{\mathbf{o}}_j}\}|}{N_{\mathbf{s}_{cr}=\bar{\mathbf{s}}_i}} \quad (36)$$

$$\leq P_{\bar{\mathbf{s}}_i}(\cup_{\mathbf{s}_{cr}^{t_k}=\bar{\mathbf{s}}_i, B(\mathbf{y}_{cr}^{t_k}, \zeta) \subset Y_{\bar{\mathbf{o}}_j}} B(\mathbf{y}_{cr}^{t_k}, \zeta)) \leq P_{\bar{\mathbf{s}}_i}(Y_{\bar{\mathbf{o}}_j}) = p^*(\mathbf{o}_{cr} = \bar{\mathbf{o}}_j | \mathbf{s}_{cr} = \bar{\mathbf{s}}_i) \quad (37)$$

For the second inequality, by definition, we obtain

$$p^{+\xi}(\mathbf{o}_{cr} = \bar{\mathbf{o}}_j | \mathbf{s}_{cr} = \bar{\mathbf{s}}_i) = \frac{|\{k | \mathbf{s}_{cr}^{t_k} = \bar{\mathbf{s}}_i, \mathbf{f}_{cr}(\bar{B}(f(\mathbf{y}_{cr}^{t_k}; \mathbf{w}_{cr}), \xi)) \supset \{\bar{\mathbf{o}}_j\}\}|}{N_{\mathbf{s}_{cr}=\bar{\mathbf{s}}_i}} \quad (38)$$

$$= 1 - \frac{|\{k | \mathbf{s}_{cr}^{t_k} = \bar{\mathbf{s}}_i, \mathbf{f}_{cr}(\bar{B}(f(\mathbf{y}_{cr}^{t_k}; \mathbf{w}_{cr}), \xi)) \subset \{\bar{\mathbf{o}}_{-j}\}\}|}{N_{\mathbf{s}_{cr}=\bar{\mathbf{s}}_i}} \quad (39)$$

when  $\bar{B}(\mathbf{y}_{cr}^{t_k}, \xi)$  denotes the closed ball centered on  $\mathbf{y}_{cr}^{t_k}$  with radius  $\xi$  and  $\{\bar{\mathbf{o}}_{-j}\}$  denotes  $\{\bar{\mathbf{o}}_1, \dots, \bar{\mathbf{o}}_{j-1}, \bar{\mathbf{o}}_{j+1}, \dots, \bar{\mathbf{o}}_{N_o}\}$ .

Then, similar to the first inequality, we can prove the second inequality based on

statements of Condition 2 as follows.

$$\begin{aligned}
p^{+\xi}(\mathbf{o}_{cr} = \bar{\mathbf{o}}_j | \mathbf{s}_{cr} = \bar{\mathbf{s}}_i) &= 1 - \frac{|\{k | \mathbf{s}_{cr}^{t_k} = \bar{\mathbf{s}}_i, \mathbf{f}_{cr}(\bar{B}(f(\mathbf{y}_{cr}^{t_k}; \mathbf{w}_{cr}), \xi)) \subset \{\bar{\mathbf{o}}_{-j}\}\}|}{N_{\mathbf{s}_{cr}=\bar{\mathbf{s}}_i}} \\
&\geq 1 - \frac{|\{k | \mathbf{s}_{cr}^{t_k} = \bar{\mathbf{s}}_i, B(\mathbf{y}_{cr}^{t_k}, \zeta) \subset \cup_{l \neq j} Y_{\bar{\mathbf{o}}_l}\}|}{N_{\mathbf{s}_{cr}=\bar{\mathbf{s}}_i}} \geq 1 - P_{\bar{\mathbf{s}}_i}(\cup_{\mathbf{s}_{cr}^{t_k}=\bar{\mathbf{s}}_i, B(\mathbf{y}_{cr}^{t_k}, \zeta) \subset \cup_{l \neq j} Y_{\bar{\mathbf{o}}_l}} B(\mathbf{y}_{cr}^{t_k}, \zeta)) \quad (40) \\
&\geq 1 - P_{\bar{\mathbf{s}}_i}(\cup_{l \neq j} Y_{\bar{\mathbf{o}}_l}) = P_{\bar{\mathbf{s}}_i}(Y_{\bar{\mathbf{o}}_j}) = p^*(\mathbf{o}_{cr} = \bar{\mathbf{o}}_j | \mathbf{s}_{cr} = \bar{\mathbf{s}}_i)
\end{aligned}$$

□

Theorem 1 implies that we can use fixed internal test cases within a safety classification model and conservative testing allows it to avoid the overfitting problem. Internal test cases, some fixed dataset separated to the training batch, can be used to design a novel AI model architecture or a novel loss function based of comparison or other calculation based on two kinds of data (training batch and internal test cases). We expect that this new (with the our best knowledge) concept to be an ingredient of a variety of novel development related to AI model.

Corollary 1 is straightforward from Theorem 1 and the definitions of the replacements of the constraints (33), (12).

**Corollary 1.** *Under Condition 1 and Condition 2,*

$$\bar{c}_i^\xi(\mathbf{u}; \mathbf{o}, \mathbf{r}) \leq \bar{c}_i^*(\mathbf{u}; \mathbf{o}, \mathbf{r}). \quad (41)$$

Now, we can formally state our main theorem as follows:

**Corollary 2.** *When the optimization problem (67) with conservative testing (when the constraints are replaced with  $\bar{c}_i^\xi$ ) have a feasible solution, it outputs the optimal solution satisfying the original constraints  $\bar{c}_i^\xi(\mathbf{u}; \mathbf{o}, \mathbf{r})$ , that is, satisfaction of safety constraints provided by the user are guaranteed.*

Now, we present the condition that makes the conservativeness of the replacement of constraints result in higher or equal loss. Since our loss function is defined separately from the optimization stage, there can be some cases where action based on conservative testing results in a smaller loss. Especially when the loss is designed to encourage conservative testing based action, it will be natural. Definition 2 that is about how the loss function well aligns with the objective of the optimization stage under a constraint.

**Definition 2.** For three functions  $\pi, \chi, \psi : R^{n_{real}} \times Z^{n_{inte}} \rightarrow R$ , we call  $\pi$  *aligns well* with  $\chi$  under constraint  $\psi \geq 0$  in set  $\mathcal{S} \subset R^{n_{real}} \times Z^{n_{inte}}$  when the following statement holds.

For all  $\alpha_1, \alpha_2 \in \mathcal{S}$ , when both  $\chi(\alpha_1) \leq \chi(\alpha_2)$  and  $\psi(\alpha_1) < 0 \leq \psi(\alpha_2)$  hold, then  $\pi(\alpha_1) \leq \pi(\alpha_2)$ .

Then, we can configure the condition that guarantees a higher loss for the conservative testing technique.

**Condition 3.** *As functions of  $\mathbf{u}$ , for any  $c_i$  needed to be replaced by chance-constrained method and any  $\bar{\mathbf{s}}_k \in \mathcal{S}_{cr}$ ,  $L(\mathbf{u}, \mathbf{o}; \bar{\mathbf{s}}_k, \mathbf{s}_{ncr}, \mathbf{r})$  aligns well with  $\bar{J}(\mathbf{u}; \mathbf{o}, \mathbf{r})$  under constraint  $c_i(\mathbf{u}; \bar{\mathbf{s}}_k, \mathbf{r}) \geq 0$  in  $\mathcal{U}$ .*

Since  $\bar{J}$  is set to obtain high control performance and  $L$  is set to evaluate the performance, it is natural to assume Condition 3. Note that Condition 3 is automatically satisfied when  $L$  is a non-decreasing function of  $\bar{J}$  or converse. Now, we can prove that the conservative testing technique results in higher or equal loss than we use the real performance value of the perception module (AI model) under the conditions.

**Proposition 3.** *Under Condition 1, Condition 2, and Condition 3, the minimum of  $L$  with the optimal action is higher or equal when the constraints are replaced with  $\bar{c}_i^\xi$  (conservative testing) than when the constraints are replaced with  $\bar{c}_i^*$  (control based on the real performance).*

*Proof.* (proof by contradiction) Suppose not. Let the optimal solution of two cases as  $\mathbf{u}_1^*, \mathbf{u}_2^*$ . Then, by the assumption,  $L(\mathbf{u}_1^*, \mathbf{o}; \bar{\mathbf{s}}_k, \mathbf{s}_{ncr}, \mathbf{r}) < L(\mathbf{u}_2^*, \mathbf{o}; \bar{\mathbf{s}}_k, \mathbf{s}_{ncr}, \mathbf{r})$ . Moreover, by Corollary 1,  $\bar{J}(\mathbf{u}_1^*; \mathbf{o}, \mathbf{r}) \geq \bar{J}(\mathbf{u}_2^*; \mathbf{o}, \mathbf{r})$  (optimal value becomes worse under stricter constraints).

Applying Condition 3 into them, we obtain that  $c_i(\mathbf{u}_1^*; \bar{\mathbf{s}}_k, \mathbf{r}) \geq 0$  implies  $c_i(\mathbf{u}_2^*; \bar{\mathbf{s}}_k, \mathbf{r}) \geq 0$  for every  $c_i$  needed to be replaced. Since its reverse holds by Theorem 1, this means that  $\mathbf{u}_1^*$  and  $\mathbf{u}_2^*$  satisfy same set of original constraints. Thus, considering that  $\mathbf{u}_1^*$  and  $\mathbf{u}_2^*$  are the optimal solutions,  $\bar{J}(\mathbf{u}_1^*; \mathbf{o}, \mathbf{r}) = \bar{J}(\mathbf{u}_2^*; \mathbf{o}, \mathbf{r})$  and this contradicts with the assumption.  $\square$

To conclude the theoretical analysis regarding conservative testing and chance-constraint, we finally present that this technique can also be included in the general framework in Section 1.

**Proposition 4.** *When both  $\mathcal{S}_{cr}$  and  $\mathcal{O}_{cr}$  are finite, our conservative testing technique for chance-constrained formulation (31),(32),(33) is included in our general framework presented in Section 1. Moreover, replacements of constraints are continuous with respect to continuous part of  $\mathbf{u}$  and  $\mathbf{o}$  provided that original constraints to be replaced are continuous with respect to continuous part of  $\mathbf{u}$ .*

*Proof.* The part for obtaining  $\mathbf{1}^{+\xi}(f(\mathbf{y}_{cr}^{tk}; \mathbf{w}_{cr}), \bar{\mathbf{o}}_j)$  or  $\mathbf{1}^{-\xi}(f(\mathbf{y}_{cr}^{tk}; \mathbf{w}_{cr}), \bar{\mathbf{o}}_j)$  can be treated as the change of the last layer of the safety classification model. Other things are the same with the proof of Proposition 1.  $\square$

## 4 Construction of the Loss function for Training

We need a *loss function* to train the AI model in our framework. First, we denote it as  $L(\mathbf{u}, \mathbf{o}; \mathbf{s}, \mathbf{r})$ . We define our loss function as a general function of  $\mathbf{u}, \mathbf{o}, \mathbf{s}$ , and  $\mathbf{r}$  that can include any kind of functions regarding them. In most cases,  $J(\mathbf{u}; \mathbf{s}, \mathbf{r})$  is used as  $L(\mathbf{u}, \mathbf{o}; \mathbf{s}, \mathbf{r})$ . Nonetheless, in our framework, the loss function can be any function of  $\mathbf{u}, \mathbf{o}, \mathbf{s}$ , and  $\mathbf{r}$ . For example, it can include the objective of the optimization stage  $\bar{J}$  or traditional loss functions based on  $\mathbf{o}$  and  $\mathbf{s}$  that are used for perception such as cross-entropy loss or root mean square loss. This can be useful when the user of our framework needs to explicitly improve the accuracy of the AI nmodel output for reasons other than the system performance.

We need to obtain the gradient of our loss function to use it for training. However, since the loss function is the function of  $\mathbf{u}$ , the loss function with the control outputs  $L(\mathbf{u}^*(\mathbf{o}, \mathbf{r}), \mathbf{o}; \mathbf{s}, \mathbf{r})$  depends on the optimal solutions of the optimization stage  $\mathbf{u}^*(\mathbf{o}, \mathbf{r})$  (called as *actions* below) that are not generally continuous functions of AI model output  $\mathbf{o}$  and it makes the gradient usually diverge or disappear (See ? for further description). Moreover, when there are multiple optimal solutions in the optimization stage, the corresponding values of the loss function can be different. One fatal problem of this is that the loss cannot be well-defined as a function of only  $\mathbf{o}, \mathbf{s}$ , and  $\mathbf{r}$ . Even though we construct a well-defined function that has a minimum value of the loss function among  $\mathbf{u}$  that is an optimal solution of the optimization stage, a similar problem remains because it requires solving a two-stage minimization (minimization in argmin set in another problem) that is computationally hard. Since we deal with general optimization problem, we cannot guarantee that we can have a closed-form solution to the optimal set of the problem. According to our best knowledge, no literature explicitly deal with the possibility of the existence of multiple optimal solutions for the optimization stage.

As an alternative of the loss function with actions  $L(\mathbf{u}^*(\mathbf{o}, \mathbf{r}), \mathbf{o}; \mathbf{s}, \mathbf{r})$ , we need to use the *approximated general loss function* denoted as  $\tilde{L}$  that is well-defined and continuous with respect of  $\mathbf{o}$  and satisfies  $\tilde{L} \simeq L(\mathbf{u}^*(\mathbf{o}, \mathbf{r}), \mathbf{o}; \mathbf{s}, \mathbf{r})$  with an action chosen by the optimization stage. Note that  $\tilde{L}$  does not have to be able to be written as a closed form. It may include some optimization problems. The only condition it needs to meet is the continuity with respect to  $\mathbf{o}$ .

Since we do not assume any specific relationship between the optimization problem and the loss function, to avoid solving the two-stage minimization (minimizing the loss function within the optimal solution set of the optimization stage in which we even might not be able to obtain the closed-form solution of the first minimization, we should combine the two stages into one stage. Before combining them later, we should solve the continuity issue. To construct the approximate loss function that is continuous, we use the property that the optimal objective of an optimization problem is continuous



with respect to parameters when the objective function is continuous with respect to the parameters and constraints are independent of the parameters. Thus, converting the optimization stage to a virtually unconstrained (constraints do not have any meaningful effect on the solution) optimization problem can be a good way for the first stage of constructing such approximated loss function that is ensuring the continuity with respect to output  $\mathbf{o}$  before combining it with the loss function. We convert the problem to an optimization problem with a compact feasible region that does not depend on any parameters by merging constraints with coefficient  $\beta > 0$  into the objective. We need the compact feasible region to prevent  $\bar{J}$  from diverging to  $-\infty$ . We can choose region  $\mathcal{U}$  with simple constraints such as  $\|\mathbf{u}\| \leq M$ . Note that we can use any norm paired with other mathematical concepts, such as compactness and continuity. The resulting converted optimization problem can be written as (42).

$$\min_{\mathbf{u} \in \mathcal{U} \subset \mathcal{X} \times \mathcal{Z}} \bar{J}(\mathbf{u}; \mathbf{o}, \mathbf{r}) - \beta^\top \min(\bar{\mathbf{c}}(\mathbf{u}; \mathbf{o}, \mathbf{r}), \mathbf{0}) \quad (42)$$

This conversion cannot guarantee the equivalence between the original and converted optimization problem because the constraints can be nearly stationary (such as local maximum or minimum point) at the boundary of the feasible region, and this leads to a solution infeasible in the original optimization problem even if  $\beta_i$  is extremely big for every  $i$ . Instead, since the output of the optimization layer is the optimal solution  $\mathbf{u}$ , we check the distance between the solutions of these two optimization problems. Considering that the loss function or the real performance mainly depends on actions instead of the optimal value in the optimization stage, the conversion is valid if and only if it leads to similar actions (optimal solutions). We aim to make the conversion have solutions sufficiently close to the original solutions under given  $\mathcal{U}$  by choosing appropriate  $\beta_i$  for all  $i$ . To guarantee that, we need both  $\bar{J}(\mathbf{u}; \mathbf{o}, \mathbf{r})$  and  $\bar{\mathbf{c}}_i(\mathbf{u}; \mathbf{o}, \mathbf{r})$  for all  $i$  are continuous with respect to  $\mathbf{x}$ . Moreover, in (42),  $\mathcal{U}$  should be a subset of  $\mathcal{X} \times \mathcal{Z}$  that only consists of finite  $\mathbf{z}$  with paired compact subsets ( $\mathcal{X}_i \subset \mathcal{X}$  for each  $z_i$ ) of  $\mathcal{X}$  and  $\cup_i \mathcal{X}_i \times \{z_i\}$  includes the region of interest. Our assumptions can be summarized as Assumption 1.

From now on, we denote the continuous part and the discrete part of  $\mathbf{u}$  as  $\mathbf{x}$  and  $\mathbf{z}$ , respectively.

**Assumption 1.**  $\bar{J}(\mathbf{u}; \mathbf{o}, \mathbf{r})$ ,  $\bar{\mathbf{c}}_i(\mathbf{u}; \mathbf{o}, \mathbf{r})$ , and  $\mathcal{U}$  satisfy the following statements.

1.  $\bar{J}(\mathbf{u}; \mathbf{o}, \mathbf{r})$  is continuous with respect to  $\mathbf{x}$ .
2. For all  $i$ ,  $\bar{\mathbf{c}}_i(\mathbf{u}; \mathbf{o}, \mathbf{r})$  is continuous with respect to  $\mathbf{x}$ .
3.  $\mathcal{U}$  is a finite union of multiplications of different elements of  $\mathcal{Z}$  and paired compact subsets of  $\mathcal{X}$ .

That is,  $\mathcal{U}$  can be written as  $\bigcup_1^{m_u(<\infty)} \mathcal{X}_i \times \{\mathbf{z}_i\}, \forall i, \mathcal{X}_i \subset \mathcal{X}: \text{compact}, \forall i, j, \mathbf{z}_i \neq \mathbf{z}_j$ .

4.  $\mathcal{U}$  includes all optimal solutions of (67).

For notational convenience, we denote the optimal solution space of the non-converted optimization problem as  $S(\mathbf{o}, \mathbf{r}) := \arg \min_{\mathbf{u}} \bar{J}(\mathbf{u}; \mathbf{o}, \mathbf{r})$  s.t.  $\bar{\mathbf{c}}(\mathbf{u}; \mathbf{o}, \mathbf{r}) \geq 0$  and solution space of  $\mathbf{x}$  paired with specific  $\mathbf{z}$  as  $S_{\mathbf{z}}(\mathbf{o}, \mathbf{r}) := \{\mathbf{x} : \mathbf{u} \in S(\mathbf{o}, \mathbf{r})\}$ . Then, Proposition 5 states that we can arbitrarily reduce the distance between solutions of the original optimization problem and the converted problem by choosing sufficiently big  $\beta$  under given  $\mathbf{o}$  and  $\mathbf{r}$ .

**Proposition 5.** *When  $\bar{J}(\mathbf{u}; \mathbf{o}, \mathbf{r})$ ,  $\bar{c}_i(\mathbf{u}; \mathbf{o}, \mathbf{r})$ , and  $\mathcal{U}$  satisfy Assumption 1, for any  $\epsilon_1 > 0$ , there exists  $\underline{\beta}(\mathbf{o}, \mathbf{r}, \epsilon_1) > 0$  s.t.,*

*any  $\beta > \underline{\beta}$  makes all solutions of the converted problem is at most at a distance  $\epsilon_1$  from a solution of the original problem with the same  $\mathbf{z}$ . That is,*

$$\begin{aligned} \forall \beta > \underline{\beta}, \forall (\tilde{\mathbf{x}}, \mathbf{z}) \in \arg \min_{\mathbf{u} \in \mathcal{U}} \bar{J}(\mathbf{u}; \mathbf{o}, \mathbf{r}) - \beta^\top \min(\bar{\mathbf{c}}(\mathbf{u}; \mathbf{o}, \mathbf{r}), \mathbf{0}), \\ \exists \mathbf{x}^*, \|\mathbf{x}^* - \tilde{\mathbf{x}}\| < \epsilon_1, \mathbf{x}^* \in S_{\mathbf{z}}(\mathbf{o}, \mathbf{r}) \end{aligned} \quad (43)$$

*Proof.* We denote the union of  $\epsilon_1$  balls (In this paper, 'a-ball' means an open ball.) centered on elements of the  $S_{\mathbf{z}}(\mathbf{o}, \mathbf{r})$  as  $\tilde{S}_{\mathbf{z}}(\mathbf{o}, \mathbf{r}, \epsilon_1) = \bigcup_{\mathbf{x} \in S_{\mathbf{z}}(\mathbf{o}, \mathbf{r})} B(\mathbf{x}, \epsilon_1)$  for all  $\mathbf{z}$  and  $\tilde{S}(\mathbf{o}, \mathbf{r}, \epsilon_1) = \bigcup_{\mathbf{z}} \tilde{S}_{\mathbf{z}}(\mathbf{o}, \mathbf{r}, \epsilon_1) \times \{\mathbf{z}\}$ . Then, for each  $\mathbf{z}$ ,  $\tilde{S}_{\mathbf{z}}(\mathbf{o}, \mathbf{r}, \epsilon_1)$  is open because it is a union of open balls. This implies that  $\mathcal{U}_{\mathbf{z}} \setminus \tilde{S}(\mathbf{o}, \mathbf{r}, \epsilon_1) (= \mathcal{U}_{\mathbf{z}} \setminus \tilde{S}_{\mathbf{z}}(\mathbf{o}, \mathbf{r}, \epsilon_1))$  is compact for  $\mathcal{U}_{\mathbf{z}} := \mathcal{U} \cap (\mathcal{X} \times \{\mathbf{z}\})$ .

Meanwhile, when we denote the optimal value of the non-converted optimization problem as  $\bar{J}^*(\mathbf{o}; \mathbf{r})$  and the set of points that lead to a smaller or equal objective than  $\bar{J}^*(\mathbf{o}; \mathbf{r})$  as  $H(\mathbf{o}, \mathbf{r}) = \{\mathbf{u} \in \mathcal{U} | \bar{J}(\mathbf{u}; \mathbf{o}, \mathbf{r}) \leq \bar{J}^*(\mathbf{o}; \mathbf{r})\}$ , it is clear that all solutions of the converted optimization problem are included in  $H(\mathbf{o}, \mathbf{r})$  regardless of  $\beta$ . Since  $\bar{J}$  is continuous,  $H(\mathbf{o}, \mathbf{r})$ , which is the inverse image of a closed set, is closed. Thus,  $\mathcal{U}_{\mathbf{z}} \cap H(\mathbf{o}, \mathbf{r})$  is an intersection of a closed set with a compact set and is thus compact. As a result,  $(\mathcal{U}_{\mathbf{z}} \cap H(\mathbf{o}, \mathbf{r})) \setminus \tilde{S}(\mathbf{o}, \mathbf{r}, \epsilon_1)$  is compact for any  $\mathbf{z}$ .

Considering that all feasible solutions (of the original problem) that are included in  $H(\mathbf{o}, \mathbf{r})$  are optimal, they are elements of  $S(\mathbf{o}, \mathbf{r})$ . It implies that all elements of  $(\mathcal{U}_{\mathbf{z}} \cap H(\mathbf{o}, \mathbf{r})) \setminus \tilde{S}(\mathbf{o}, \mathbf{r}, \epsilon_1)$  make at least one of the constraints violated. Then, we can construct  $\phi(\mathbf{u}; \mathbf{o}, \mathbf{r}) : (\mathcal{U}_{\mathbf{z}} \cap H(\mathbf{o}, \mathbf{r})) \setminus \tilde{S}(\mathbf{o}, \mathbf{r}, \epsilon_1) \rightarrow \mathbb{R}^+$ ,  $\phi(\mathbf{u}; \mathbf{o}, \mathbf{r}) = \frac{\bar{J}(\mathbf{u}; \mathbf{o}, \mathbf{r}) - \bar{J}^*(\mathbf{o}; \mathbf{r})}{\min_i \bar{c}_i(\mathbf{u}; \mathbf{o}, \mathbf{r})}$ . Note that  $\phi(\mathbf{u}; \mathbf{o}, \mathbf{r})$  is not a function of  $\epsilon_1$ . Finally, since  $\phi(\mathbf{u}; \mathbf{o}, \mathbf{r})$  is the ratio of two continuous functions thus continuous, we can choose the maximum value of  $\phi(\mathbf{u}; \mathbf{o}, \mathbf{r})$  due to the compactness of  $(\mathcal{U}_{\mathbf{z}} \cap H(\mathbf{o}, \mathbf{r})) \setminus \tilde{S}(\mathbf{o}, \mathbf{r}, \epsilon_1)$ .

Let us denote the maximum value of  $\phi(\mathbf{u}; \mathbf{o}, \mathbf{r})$  with respect to  $\mathbf{x}$  as  $\mu(\mathbf{z}; \mathbf{o}, \mathbf{r}, \epsilon_1)$  and  $\underline{\beta}(\mathbf{o}, \mathbf{r}, \epsilon_1) := \max_{\mathbf{z}} \mu(\mathbf{z}; \mathbf{o}, \mathbf{r}, \epsilon_1) \mathbf{1}$ . Then  $\forall \beta > \underline{\beta}$  and  $\forall \mathbf{z} \in \mathcal{Z}$ , for any elements

of  $(\mathcal{U}_{\mathbf{z}} \cap H(\mathbf{o}, \mathbf{r})) \setminus \tilde{S}(\mathbf{o}, \mathbf{r}, \epsilon_1)$ , we have

$$\begin{aligned}
& \bar{J}(\mathbf{u}; \mathbf{o}, \mathbf{r}) - \beta^\top \min(\bar{\mathbf{c}}(\mathbf{u}; \mathbf{o}, \mathbf{r}), \mathbf{0}) \\
& > \bar{J}(\mathbf{u}; \mathbf{o}, \mathbf{r}) - \max_{\mathbf{z}'} \mu(\mathbf{z}'; \mathbf{o}, \mathbf{r}, \epsilon_1) \mathbf{1}^\top \min(\bar{\mathbf{c}}(\mathbf{u}; \mathbf{o}, \mathbf{r}), \mathbf{0}) \\
& \geq \bar{J}(\mathbf{u}; \mathbf{o}, \mathbf{r}) - \mu(\mathbf{z}; \mathbf{o}, \mathbf{r}, \epsilon_1) \mathbf{1}^\top \min(\bar{\mathbf{c}}(\mathbf{u}; \mathbf{o}, \mathbf{r}), \mathbf{0}) \\
& \geq \bar{J}(\mathbf{u}; \mathbf{o}, \mathbf{r}) - \frac{\bar{J}(\mathbf{u}; \mathbf{o}, \mathbf{r}) - \bar{J}^*(\mathbf{o}; \mathbf{r})}{\min_i \bar{c}_i(\mathbf{u}; \mathbf{o}, \mathbf{r})} \mathbf{1}^\top \min(\bar{\mathbf{c}}(\mathbf{u}; \mathbf{o}, \mathbf{r}), \mathbf{0}) \\
& = \bar{J}(\mathbf{u}; \mathbf{o}, \mathbf{r}) - (\bar{J}(\mathbf{u}; \mathbf{o}, \mathbf{r}) - \bar{J}^*(\mathbf{o}; \mathbf{r})) \sum_j \frac{\min(\bar{c}_j(\mathbf{u}; \mathbf{o}, \mathbf{r}), 0)}{\min_i \bar{c}_i(\mathbf{u}; \mathbf{o}, \mathbf{r})} \geq \bar{J}^*(\mathbf{o}; \mathbf{r}).
\end{aligned} \tag{44}$$

Note that  $\beta^\top \min(\bar{\mathbf{c}}(\mathbf{u}; \mathbf{o}, \mathbf{r}), \mathbf{0})$  is always nonpositive. The first inequality is based on the definition of  $\underline{\beta}$ . The third inequality is based on the definition of  $\mu$ . The last inequality holds because  $\bar{J}(\mathbf{u}; \mathbf{o}, \mathbf{r}) - \bar{J}^*(\mathbf{o}; \mathbf{r}) \leq 0$  in  $H(\mathbf{o}, \mathbf{r})$  and  $\min_i \bar{c}_i(\mathbf{u}; \mathbf{o}, \mathbf{r}) < 0$  due to the definition of  $H(\mathbf{o}, \mathbf{r})$  and the optimality of  $\bar{J}^*(\mathbf{o}; \mathbf{r})$ . Thus, all elements of  $(\mathcal{U}_{\mathbf{z}} \cap H(\mathbf{o}, \mathbf{r})) \setminus \tilde{S}(\mathbf{o}, \mathbf{r}, \epsilon_1)$  cannot be a solution of the converted optimization problem. Considering that all solutions of the converted optimization problem are included in  $H(\mathbf{o}, \mathbf{r})$ , all solutions of the converted optimization problem are included in  $\tilde{S}(\mathbf{o}, \mathbf{r}, \epsilon_1)$  and this implies (43).  $\square$

This conversion allows us to use the continuity of the optimal objective, provided that the objective function is continuous for both the variables and parameters. Now, similar to ?, we can construct the general approximate loss function  $\tilde{L}(\mathbf{o}; \mathbf{s}, \mathbf{r}, \beta, \lambda)$  with the converted optimization problem as follows.

$$\begin{aligned}
\tilde{L}(\mathbf{o}; \mathbf{s}, \mathbf{r}, \beta, \lambda) = & \frac{1}{\lambda} (\min_{\mathbf{u} \in \mathcal{U}} (\lambda L(\mathbf{u}, \mathbf{o}; \mathbf{s}, \mathbf{r}) + \bar{J}(\mathbf{u}; \mathbf{o}, \mathbf{r}) - \beta^\top \min(\bar{\mathbf{c}}(\mathbf{u}; \mathbf{o}, \mathbf{r}), \mathbf{0}))) \\
& - \min_{\mathbf{u} \in \mathcal{U}} (\bar{J}(\mathbf{u}; \mathbf{o}, \mathbf{r}) - \beta^\top \min(\bar{\mathbf{c}}(\mathbf{u}; \mathbf{o}, \mathbf{r}), \mathbf{0})))
\end{aligned} \tag{45}$$

We need to assume that the objective, the constraints, and the loss are continuous with respect to the variable  $\mathbf{x}$  and the parameters conveyed by the AI model  $\mathbf{o}$ . Assumption 2 covers statements we need to assume but are not covered in Assumption 1.

**Assumption 2.**  $\bar{J}(\mathbf{u}; \mathbf{o}, \mathbf{r})$ ,  $\bar{\mathbf{c}}(\mathbf{u}; \mathbf{o}, \mathbf{r})$ , and  $L(\mathbf{u}, \mathbf{o}; \mathbf{s}, \mathbf{r})$  satisfy the following statements.

1.  $\bar{J}(\mathbf{u}; \mathbf{o}, \mathbf{r})$  is continuous with respect to  $\mathbf{o}$ .
2. For all  $i$ ,  $\bar{c}_i(\mathbf{u}; \mathbf{o}, \mathbf{r})$  is continuous with respect to  $\mathbf{o}$ .
3.  $L(\mathbf{u}, \mathbf{o}; \mathbf{s}, \mathbf{r})$  is continuous with respect to  $\mathbf{x}$  and  $\mathbf{o}$ .

**Remark 1.** The third statement is about continuity of  $L(\mathbf{u}, \mathbf{o}; \mathbf{s}, \mathbf{r})$  with respect to  $\mathbf{x}$ ,  $\mathbf{o}$  as a function of  $\mathbf{u}$ , and  $\mathbf{o}$ . This is different from the continuity of  $L(\mathbf{u}^*(\mathbf{o}, \mathbf{r}), \mathbf{o}; \mathbf{s}, \mathbf{r})$  with respect to  $\mathbf{o}$  as a function of  $\mathbf{o}$ , which does not generally hold.

Under Assumption 2, we can induce the desired properties (continuous with respect to  $\mathbf{o}$  and convergence to real loss) of our approximated loss in the following theorem.

Before the proof, we define  $L^*(\mathbf{o}; \mathbf{s}, \mathbf{r})$  as below.

$$L^*(\mathbf{o}; \mathbf{s}, \mathbf{r}) := \min_{\mathbf{u} \in S(\mathbf{o}, \mathbf{r})} L(\mathbf{u}, \mathbf{o}; \mathbf{s}, \mathbf{r}) \quad (46)$$

The minimum of  $L$  is well-defined under Assumption 2 because  $S_z(\mathbf{o}, \mathbf{r})$  is compact (see the proof of Proposition 5) and  $L$  is continuous with respect to  $\mathbf{x}$ . As noted early, direct calculation of (46) is computationally hard. Instead, we prove that our approximated loss function  $\tilde{L}(\mathbf{o}; \mathbf{s}, \mathbf{r}, \boldsymbol{\beta}, \lambda)$  approaches to  $L^*(\mathbf{o}; \mathbf{s}, \mathbf{r})$  when  $\boldsymbol{\beta}$  becomes sufficiently big and  $\lambda$  becomes sufficiently small.

**Theorem 2.** *When  $\bar{J}(\mathbf{u}; \mathbf{o}, \mathbf{r}), \bar{\mathbf{c}}(\mathbf{u}; \mathbf{o}, \mathbf{r}), \mathcal{U}, L(\mathbf{u}, \mathbf{o}; \mathbf{s}, \mathbf{r})$  satisfies Assumption 1 and Assumption 2,*

*for any  $(\mathbf{o}, \mathbf{s}, \mathbf{r})$  and  $\epsilon_2 > 0$ , two following statements hold.*

1.  *$\tilde{L}(\mathbf{o}; \mathbf{s}, \mathbf{r}, \boldsymbol{\beta}, \lambda)$  is continuous with respect to (the continuous part of)  $\mathbf{o}$  for any  $\boldsymbol{\beta}(> \mathbf{0})$  and  $\lambda(> 0)$ .*
2. *We can find  $(\boldsymbol{\beta}_0(\mathbf{o}, \mathbf{r}, \lambda, \mathbf{s}, \epsilon_2), \lambda_0(\mathbf{o}, \mathbf{r}, \mathbf{s}, \epsilon_2))$  that makes any  $(\boldsymbol{\beta} > \boldsymbol{\beta}_0(\mathbf{o}, \mathbf{r}, \lambda, \mathbf{s}, \epsilon_2), \lambda < \lambda_0(\mathbf{o}, \mathbf{r}, \mathbf{s}, \epsilon_2))$  guarantees  $|\tilde{L}(\mathbf{o}; \mathbf{s}, \mathbf{r}, \boldsymbol{\beta}, \lambda) - L^*(\mathbf{o}; \mathbf{s}, \mathbf{r})| < \epsilon_2$ .*

*Proof.* At first, for any  $\boldsymbol{\beta}(> \mathbf{0})$  and  $\lambda(> 0)$ , both  $\min_{\mathbf{u} \in \mathcal{U}} (\lambda L(\mathbf{u}, \mathbf{o}; \mathbf{s}, \mathbf{r}) + \bar{J}(\mathbf{u}; \mathbf{o}, \mathbf{r}) + \boldsymbol{\beta}^\top \min(\bar{\mathbf{c}}(\mathbf{u}; \mathbf{o}, \mathbf{r}), \mathbf{0}))$  and  $\min_{\mathbf{u} \in \mathcal{U}} (\bar{J}(\mathbf{u}; \mathbf{o}, \mathbf{r}) + \boldsymbol{\beta}^\top \min(\bar{\mathbf{c}}(\mathbf{u}; \mathbf{o}, \mathbf{r}), \mathbf{0}))$  are continuous with respect to the continuous part of  $\mathbf{o}$  since they are minimal value of a continuous function with respect to  $\mathbf{x}, \mathbf{z}$ , and the continuous part of  $\mathbf{o}$  for a fixed compact set. Thus,  $\tilde{L}(\mathbf{o}; \mathbf{s}, \mathbf{r}, \boldsymbol{\beta}, \lambda)$  is continuous with respect to the continuous part of  $\mathbf{o}$ .

We define a *preferred optimal solution* of the optimization stage (67) as an optimal solution of (46) and denote the set of preferred optimal solutions as  $S^*(\mathbf{o}, \mathbf{s}, \mathbf{r})$ . Moreover, we can define *integrated optimization layer* as equation (47).

$$\min_{\mathbf{u} \in \mathcal{U}} \quad \lambda L(\mathbf{u}, \mathbf{o}; \mathbf{s}, \mathbf{r}) + \bar{J}(\mathbf{u}; \mathbf{o}, \mathbf{r}) \quad (47a)$$

$$\text{subject to} \quad \bar{c}_i(\mathbf{u}; \mathbf{o}, \mathbf{r}) \geq 0, \quad i = 1, \dots, \bar{n}_c \quad (47b)$$

Proof of the second statement consists of two steps. The first step is finding  $\lambda_0(\mathbf{o}, \mathbf{r}, \mathbf{s}, \epsilon_2)(> 0)$  that makes  $|\lambda L(\mathbf{u}^*, \mathbf{o}; \mathbf{s}, \mathbf{r}) + \bar{J}(\mathbf{x}^*, \mathbf{z}^*; \mathbf{o}, \mathbf{r}) - \lambda L^*(\mathbf{o}; \mathbf{s}, \mathbf{r}) - \bar{J}^*(\mathbf{o}; \mathbf{r})| < \frac{\lambda \epsilon_2}{3}$  for all  $\lambda < \lambda_0(\mathbf{o}, \mathbf{r}, \mathbf{s}, \epsilon_2)$  when  $\bar{J}^*(\mathbf{o}; \mathbf{r})$  is the optimal value of the original optimization stage (67) and  $(\mathbf{x}^*, \mathbf{z}^*)$  is an optimal solution of the integrated optimization layer (47). The second step is finding  $\boldsymbol{\beta}_0(\mathbf{o}, \mathbf{r}, \lambda, \mathbf{s}, \epsilon_2)$  that guarantees the minimum value of the first minimization problem of (45) and the minimal value of the second minimization problem have distance less than  $\frac{\lambda \epsilon_2}{3}$  from the minimal value of (47), (67), respectively.

Step 1. Since  $L$  is a continuous function with respect to  $\mathbf{x}$  and  $\mathcal{U}_{\mathbf{z}}$  is compact for all  $\mathbf{z}$ ,  $L$  is uniformly continuous in  $\mathcal{U}_{\mathbf{z}}$  for all  $\mathbf{z}$  and we can choose  $\delta_1(\mathbf{o}, \mathbf{s}, \mathbf{r}, \epsilon_2)$  that makes all  $\mathbf{x}_1, \mathbf{x}_2, \mathbf{z}$  satisfies that  $\|\mathbf{x}_1 - \mathbf{x}_2\| < \delta_1$  implies  $|L(\mathbf{x}_1, \mathbf{z}, \mathbf{o}; \mathbf{s}, \mathbf{r}) - L(\mathbf{x}_2, \mathbf{z}, \mathbf{o}; \mathbf{s}, \mathbf{r})| < \frac{\epsilon_2}{3}$ .

We denote  $S_{\mathbf{z}}^*(\mathbf{o}, \mathbf{s}, \mathbf{r}) := \{\mathbf{x} : \mathbf{u} \in S^*(\mathbf{o}, \mathbf{s}, \mathbf{r})\}$ . We fix a discrete variable  $\mathbf{z}$  and further denote  $\tilde{S}_{\mathbf{z}}^*(\mathbf{o}, \mathbf{s}, \mathbf{r}, \delta_1)$  as the union of  $\delta_1$ -balls centered on elements of  $S_{\mathbf{z}}^*(\mathbf{o}, \mathbf{s}, \mathbf{r})$ . Then, by the same reason as explained in Proposition 5,  $\mathcal{U}_{\mathbf{z}} \setminus \tilde{S}_{\mathbf{z}}^*(\mathbf{o}, \mathbf{s}, \mathbf{r}, \delta_1)$  is compact. Since  $L$  is continuous with respect to  $\mathbf{x}$ , we can find the minimum value of  $L$  in the intersection of the two compact sets,  $S_{\mathbf{z}}(\mathbf{o}, \mathbf{r}) \setminus \tilde{S}_{\mathbf{z}}^*(\mathbf{o}, \mathbf{s}, \mathbf{r}, \delta_1) = (\mathcal{U}_{\mathbf{z}} \cap S(\mathbf{o}, \mathbf{r})) \setminus \tilde{S}_{\mathbf{z}}^*(\mathbf{o}, \mathbf{s}, \mathbf{r}, \delta_1)$ . Let  $l(\mathbf{o}, \mathbf{s}, \mathbf{r}, \delta_1) (> L^*(\mathbf{o}; \mathbf{s}, \mathbf{r}))$  denote this minimum. By the uniform continuity, we can find  $\bar{\delta}_1$  that makes all  $\mathbf{x}_1, \mathbf{x}_2, \mathbf{z}$  satisfies that  $\|\mathbf{x}_1 - \mathbf{x}_2\| < \bar{\delta}_1$  implies  $|L(\mathbf{x}_1, \mathbf{z}, \mathbf{o}; \mathbf{s}, \mathbf{r}) - L(\mathbf{x}_2, \mathbf{z}, \mathbf{o}; \mathbf{s}, \mathbf{r})| < l(\mathbf{o}, \mathbf{s}, \mathbf{r}, \delta_1) - L^*(\mathbf{o}; \mathbf{s}, \mathbf{r})$ . Letting  $\tilde{V}_{\mathbf{z}}(\mathbf{o}, \mathbf{s}, \mathbf{r}, \bar{\delta}_1)$  as the union of  $\bar{\delta}_1$ -balls centered on elements of  $S_{\mathbf{z}}(\mathbf{o}, \mathbf{r}) \setminus \tilde{S}_{\mathbf{z}}^*(\mathbf{o}, \mathbf{s}, \mathbf{r}, \delta_1)$ , it is guaranteed that all elements of  $\tilde{V}_{\mathbf{z}}(\mathbf{o}, \mathbf{s}, \mathbf{r}, \bar{\delta}_1)$  have  $L$  value bigger than  $L^*(\mathbf{o}; \mathbf{s}, \mathbf{r})$ . Note that our preferred optimal solutions, which are also feasible solutions of not only the original optimization problem but also our integrated optimization layer (47), have  $\bar{J}^*(\mathbf{o}; \mathbf{r})$  and  $L^*(\mathbf{o}; \mathbf{s}, \mathbf{r})$  as the value of  $\bar{J}$  and  $L$ . Since no feasible solution of the integrated optimization layer (47) can have  $\bar{J}$  value smaller than  $\bar{J}^*(\mathbf{o}; \mathbf{r})$  because they are also the feasible solution of the original optimal solution, any element of  $\tilde{V}_{\mathbf{z}}(\mathbf{o}, \mathbf{s}, \mathbf{r}, \bar{\delta}_1)$  regardless of  $\lambda$ , is strongly dominated by all preferred optimal solutions, and thus, cannot be an optimal solution of the integrated optimization layer (47) since they have bigger  $L$  value than other feasible solution (preferred optimal solution) of the integrated optimization layer.

It is clear that  $\mathcal{U}_{\mathbf{z}} \setminus \tilde{V}_{\mathbf{z}}(\mathbf{o}, \mathbf{s}, \mathbf{r}, \bar{\delta}_1)$  is compact and thus  $(\mathcal{U}_{\mathbf{z}} \setminus \tilde{S}_{\mathbf{z}}^*(\mathbf{o}, \mathbf{s}, \mathbf{r}, \delta_1)) \setminus \tilde{V}_{\mathbf{z}}(\mathbf{o}, \mathbf{s}, \mathbf{r}, \bar{\delta}_1)$  is also compact. Moreover, since all constraints are continuous with respect to  $\mathbf{x}$ , letting the set of feasible solutions denote as  $F(\mathbf{o}, \mathbf{r})$ ,  $F(\mathbf{o}, \mathbf{r})$  is an intersection of constraint-satisfaction regions of each constraint. Since each constraint include equality, the constraint-satisfaction region is a continuous inverse image of a closed set and thus closed. Then,  $F(\mathbf{o}, \mathbf{r})$  is also closed and  $\mathcal{U}_{\mathbf{z}} \cap F(\mathbf{o}, \mathbf{r})$  is compact for all  $\mathbf{z}$ . Next, we can find the minimum value of  $\bar{J}$  in the intersection of the two compact sets,  $((\mathcal{U}_{\mathbf{z}} \cap F(\mathbf{o}, \mathbf{r})) \setminus \tilde{S}_{\mathbf{z}}^*(\mathbf{o}, \mathbf{s}, \mathbf{r}, \delta_1)) \setminus \tilde{V}_{\mathbf{z}}(\mathbf{o}, \mathbf{s}, \mathbf{r}, \bar{\delta}_1)$ . Let  $q_0(\mathbf{z}, \mathbf{o}, \mathbf{s}, \mathbf{r}, \delta_1)$  denotes the minimum value. (Note that  $\bar{\delta}_1$  is a function of  $\mathbf{z}, \mathbf{o}, \mathbf{s}, \mathbf{r}, \delta_1$ .) We can also find the maximum value  $\bar{l}(\mathbf{z}, \mathbf{o}, \mathbf{r}, \mathbf{s}, \delta_1)$  and the minimum value  $\underline{l}(\mathbf{z}, \mathbf{o}, \mathbf{r}, \mathbf{s}, \delta_1)$  of  $L(\mathbf{u}, \mathbf{o}; \mathbf{s}, \mathbf{r})$  in  $\mathcal{U}_{\mathbf{z}} \cap F(\mathbf{o}, \mathbf{r})$  because  $L(\mathbf{u}, \mathbf{o}; \mathbf{s}, \mathbf{r})$  is continuous with respect to  $\mathbf{x}$ . Thus, when we let  $\underline{\lambda}_{\mathbf{z}}(\mathbf{o}, \mathbf{r}, \mathbf{s}, \epsilon_2) := \frac{q_0(\mathbf{z}, \mathbf{o}, \mathbf{s}, \mathbf{r}, \delta_1) - \bar{J}^*(\mathbf{o}; \mathbf{r})}{\bar{l}(\mathbf{z}, \mathbf{o}, \mathbf{r}, \mathbf{s}, \delta_1) - \underline{l}(\mathbf{z}, \mathbf{o}, \mathbf{r}, \mathbf{s}, \delta_1)}$  and  $\underline{\lambda}(\mathbf{o}, \mathbf{r}, \mathbf{s}, \epsilon_2) := \min_{\mathbf{z} \in \text{Proj}_{\mathbf{Z}}(\mathcal{U})} \underline{\lambda}_{\mathbf{z}}(\mathbf{o}, \mathbf{r}, \mathbf{s}, \epsilon_2)$ , for any positive  $\lambda < \underline{\lambda}(\mathbf{o}, \mathbf{r}, \mathbf{s}, \epsilon_2)$ , there is no solution of the integrated optimization problem (47) in  $((\mathcal{U}_{\mathbf{z}} \cap F(\mathbf{o}, \mathbf{r})) \setminus \tilde{S}_{\mathbf{z}}^*(\mathbf{o}, \mathbf{s}, \mathbf{r}, \delta_1)) \setminus \tilde{V}_{\mathbf{z}}(\mathbf{o}, \mathbf{s}, \mathbf{r}, \bar{\delta}_1)$ . Since any element of  $\tilde{V}_{\mathbf{z}}(\mathbf{o}, \mathbf{s}, \mathbf{r}, \bar{\delta}_1)$  cannot be an optimal solution of (47), all optimal solutions of (47) are elements of  $\tilde{S}_{\mathbf{z}}^*(\mathbf{o}, \mathbf{s}, \mathbf{r}, \delta_1)$  for some  $\mathbf{z}$ , that is, all of them are at most in distance  $\delta_1$  from a preferred optimal solution of the original optimization stage (67) that have  $L^*(\mathbf{o}; \mathbf{s}, \mathbf{r})$  and  $\bar{J}^*(\mathbf{o}; \mathbf{r})$  as values of  $L$  and  $\bar{J}$ , respectively. Thus, we can obtain the inequalities below. Inequalities below are based on triangle inequalities and hold for any

$\lambda$  including negative numbers.

$$\begin{aligned}
\min_{\mathbf{u} \in F(\mathbf{o}, \mathbf{r})} (\lambda L(\mathbf{u}, \mathbf{o}; \mathbf{s}, \mathbf{r}) + \bar{J}(\mathbf{u}; \mathbf{o}, \mathbf{r})) &= \min_{\mathbf{u} \in \tilde{S}_{\mathbf{z}}^*(\mathbf{o}, \mathbf{s}, \mathbf{r}, \delta_1)} (\lambda L(\mathbf{u}, \mathbf{o}; \mathbf{s}, \mathbf{r}) + \bar{J}(\mathbf{u}; \mathbf{o}, \mathbf{r})) \\
&\geq \min_{\mathbf{u} \in \tilde{S}_{\mathbf{z}}^*(\mathbf{o}, \mathbf{s}, \mathbf{r}, \delta_1)} \lambda L(\mathbf{u}, \mathbf{o}; \mathbf{s}, \mathbf{r}) + \min_{\mathbf{u} \in \tilde{S}_{\mathbf{z}}^*(\mathbf{o}, \mathbf{s}, \mathbf{r}, \delta_1)} \bar{J}(\mathbf{u}; \mathbf{o}, \mathbf{r}) \quad (48) \\
&= \min_{\mathbf{u} \in \tilde{S}_{\mathbf{z}}^*(\mathbf{o}, \mathbf{s}, \mathbf{r}, \delta_1)} \lambda L(\mathbf{u}, \mathbf{o}; \mathbf{s}, \mathbf{r}) + \bar{J}^*(\mathbf{o}; \mathbf{r}) \\
\min_{\mathbf{u} \in F(\mathbf{o}, \mathbf{r})} (\lambda L(\mathbf{u}, \mathbf{o}; \mathbf{s}, \mathbf{r}) + \bar{J}(\mathbf{u}; \mathbf{o}, \mathbf{r})) &= \min_{\mathbf{u} \in \tilde{S}_{\mathbf{z}}^*(\mathbf{o}, \mathbf{s}, \mathbf{r}, \delta_1)} (\lambda L(\mathbf{u}, \mathbf{o}; \mathbf{s}, \mathbf{r}) + \bar{J}(\mathbf{u}; \mathbf{o}, \mathbf{r})) \\
&= - \min_{\mathbf{u} \in \tilde{S}_{\mathbf{z}}^*(\mathbf{o}, \mathbf{s}, \mathbf{r}, \delta_1)} (-\lambda L(\mathbf{u}, \mathbf{o}; \mathbf{s}, \mathbf{r})) + \min_{\mathbf{u} \in \tilde{S}_{\mathbf{z}}^*(\mathbf{o}, \mathbf{s}, \mathbf{r}, \delta_1)} (-\lambda L(\mathbf{u}, \mathbf{o}; \mathbf{s}, \mathbf{r})) \\
&\quad + \min_{\mathbf{u} \in \tilde{S}_{\mathbf{z}}^*(\mathbf{o}, \mathbf{s}, \mathbf{r}, \delta_1)} (\lambda L(\mathbf{u}, \mathbf{o}; \mathbf{s}, \mathbf{r}) + \bar{J}(\mathbf{u}; \mathbf{o}, \mathbf{r})) \\
&= \max_{\mathbf{u} \in \tilde{S}_{\mathbf{z}}^*(\mathbf{o}, \mathbf{s}, \mathbf{r}, \delta_1)} \lambda L(\mathbf{u}, \mathbf{o}; \mathbf{s}, \mathbf{r}) + \min_{\mathbf{u} \in \tilde{S}_{\mathbf{z}}^*(\mathbf{o}, \mathbf{s}, \mathbf{r}, \delta_1)} (-\lambda L(\mathbf{u}, \mathbf{o}; \mathbf{s}, \mathbf{r})) \\
&\quad + \min_{\mathbf{u} \in \tilde{S}_{\mathbf{z}}^*(\mathbf{o}, \mathbf{s}, \mathbf{r}, \delta_1)} (\lambda L(\mathbf{u}, \mathbf{o}; \mathbf{s}, \mathbf{r}) + \bar{J}(\mathbf{u}; \mathbf{o}, \mathbf{r})) \\
&\leq \max_{\mathbf{u} \in \tilde{S}_{\mathbf{z}}^*(\mathbf{o}, \mathbf{s}, \mathbf{r}, \delta_1)} \lambda L(\mathbf{u}, \mathbf{o}; \mathbf{s}, \mathbf{r}) + \min_{\mathbf{u} \in \tilde{S}_{\mathbf{z}}^*(\mathbf{o}, \mathbf{s}, \mathbf{r}, \delta_1)} (-\lambda L(\mathbf{u}, \mathbf{o}; \mathbf{s}, \mathbf{r}) + \lambda L(\mathbf{u}, \mathbf{o}; \mathbf{s}, \mathbf{r}) + \bar{J}(\mathbf{u}; \mathbf{o}, \mathbf{r})) \\
&\quad = \max_{\mathbf{u} \in \tilde{S}_{\mathbf{z}}^*(\mathbf{o}, \mathbf{s}, \mathbf{r}, \delta_1)} \lambda L(\mathbf{u}, \mathbf{o}; \mathbf{s}, \mathbf{r}) + \min_{\mathbf{u} \in \tilde{S}_{\mathbf{z}}^*(\mathbf{o}, \mathbf{s}, \mathbf{r}, \delta_1)} \bar{J}(\mathbf{u}; \mathbf{o}, \mathbf{r}) \\
&\quad = \max_{\mathbf{u} \in \tilde{S}_{\mathbf{z}}^*(\mathbf{o}, \mathbf{s}, \mathbf{r}, \delta_1)} \lambda L(\mathbf{u}, \mathbf{o}; \mathbf{s}, \mathbf{r}) + \bar{J}^*(\mathbf{o}; \mathbf{r}) \quad (49)
\end{aligned}$$

Therefore, considering the definition of  $\delta_1$  and  $\tilde{S}_{\mathbf{z}}^*(\mathbf{o}, \mathbf{s}, \mathbf{r}, \delta_1)$ , we obtain that any optimal solution  $\mathbf{u}^*$  of (47) satisfy  $|\lambda L(\mathbf{u}^*, \mathbf{o}; \mathbf{s}, \mathbf{r}) + \bar{J}(\mathbf{x}^*, \mathbf{z}^*; \mathbf{o}, \mathbf{r}) - \lambda L^*(\mathbf{o}; \mathbf{s}, \mathbf{r}) - \bar{J}^*(\mathbf{o}; \mathbf{r})| < \frac{\lambda \epsilon_2}{3}$ .

Step 2. Now, we fix  $\lambda$  and find  $\beta_0$  that makes the minimum value of the first and the second minimization problem of (45) have distance less than  $\frac{\lambda \epsilon_2}{3}$  from the minimal value of their constrained (unconverted) versions. By Assumption 1 and Assumption 2, both  $\lambda L(\mathbf{u}, \mathbf{o}; \mathbf{s}, \mathbf{r}) + \bar{J}(\mathbf{u}; \mathbf{o}, \mathbf{r})$  and  $\bar{J}(\mathbf{u}; \mathbf{o}, \mathbf{r})$  are continuous with respect to  $\mathbf{x}$  and our domain with respect to  $\mathbf{x}$  can be restricted to a compact set for any  $\mathbf{z}$ . Then, those two functions are uniformly continuous and we can find  $\delta_2(\mathbf{o}, \mathbf{s}, \mathbf{r}, \epsilon_2, \lambda)$  and  $\delta_3(\mathbf{o}, \mathbf{r}, \epsilon_2, \lambda)$  that make all  $\mathbf{x}_1, \mathbf{x}_2, \mathbf{z}$  satisfies that  $\|\mathbf{x}_1 - \mathbf{x}_2\| < \delta_2(\mathbf{o}, \mathbf{s}, \mathbf{r}, \epsilon_2, \lambda)$  implies  $|\lambda L(\mathbf{x}_1, \mathbf{z}, \mathbf{o}; \mathbf{s}, \mathbf{r}) + \bar{J}(\mathbf{x}_1, \mathbf{z}; \mathbf{o}, \mathbf{r}) - \lambda L(\mathbf{x}_2, \mathbf{z}, \mathbf{o}; \mathbf{s}, \mathbf{r}) - \bar{J}(\mathbf{x}_2, \mathbf{z}; \mathbf{o}, \mathbf{r})| < \frac{\lambda \epsilon_2}{3}$  and  $\|\mathbf{x}_1 - \mathbf{x}_2\| < \delta_3(\mathbf{o}, \mathbf{r}, \epsilon_2, \lambda)$  implies  $|\bar{J}(\mathbf{x}_1, \mathbf{z}; \mathbf{o}, \mathbf{r}) - \bar{J}(\mathbf{x}_2, \mathbf{z}; \mathbf{o}, \mathbf{r})| < \frac{\lambda \epsilon_2}{3}$ . Since we can treat  $\lambda L(\mathbf{u}, \mathbf{o}; \mathbf{s}, \mathbf{r}) + \bar{J}(\mathbf{u}; \mathbf{o}, \mathbf{r})$  as another  $\bar{J}$  and it satisfies Assumption 1 ( $\bar{c}$  and  $\mathcal{U}$  are same and still satisfies Assumption 1) we can apply Proposition 5 to both (47) and (67). Thus, we can choose  $\underline{\beta}_1(\mathbf{o}, \mathbf{s}, \mathbf{r}, \epsilon_2, \lambda)$  and  $\underline{\beta}_2(\mathbf{o}, \mathbf{r}, \epsilon_2)$  that make  $\beta > \underline{\beta}_1(\mathbf{u}, \mathbf{o}, \mathbf{s}, \mathbf{r}, \epsilon_2, \lambda)$  implies the optimal solution of the first minimization problem of (45) have distance less than  $\delta_2(\mathbf{o}, \mathbf{s}, \mathbf{r}, \epsilon_2, \lambda)$  from an optimal solution of (47) and  $\beta > \underline{\beta}_2(\mathbf{u}, \mathbf{o}, \mathbf{r}, \epsilon_2)$  implies the optimal solution of the second minimization problem of (45) have distance less than  $\delta_3(\mathbf{o}, \mathbf{r}, \epsilon_2)$  from an optimal solution of (67). Finally, when we set  $\beta_0(\mathbf{o}, \mathbf{r}, \lambda, \mathbf{s}, \epsilon_2) = \max(\underline{\beta}_1(\mathbf{o}, \mathbf{s}, \mathbf{r}, \epsilon_2, \lambda), \underline{\beta}_2(\mathbf{o}, \mathbf{r}, \epsilon_2))$ , all

$\beta > \beta_0(\mathbf{o}, \mathbf{r}, \lambda, \mathbf{s}, \epsilon_2)$  satisfy the following equation.

$$\begin{aligned}
& \lambda |\tilde{L}(\mathbf{o}; \mathbf{s}, \mathbf{r}, \beta, \lambda) - L^*(\mathbf{o}; \mathbf{s}, \mathbf{r})| \\
&= |\min_{\mathbf{u} \in \mathcal{U}} (\lambda L(\mathbf{u}, \mathbf{o}; \mathbf{s}, \mathbf{r}) + \bar{J}(\mathbf{u}; \mathbf{o}, \mathbf{r}) - \beta^\top \min(\bar{\mathbf{c}}(\mathbf{u}; \mathbf{o}, \mathbf{r}), \mathbf{0})) \\
&\quad - \min_{\mathbf{u} \in \mathcal{U}} (\bar{J}(\mathbf{u}; \mathbf{o}, \mathbf{r}) - \beta^\top \min(\bar{\mathbf{c}}(\mathbf{u}; \mathbf{o}, \mathbf{r}), \mathbf{0})) - \lambda L^*(\mathbf{o}; \mathbf{s}, \mathbf{r})| \\
&= |(\min_{\mathbf{u} \in \mathcal{U}} (\lambda L(\mathbf{u}, \mathbf{o}; \mathbf{s}, \mathbf{r}) + \bar{J}(\mathbf{u}; \mathbf{o}, \mathbf{r}) - \beta^\top \min(\bar{\mathbf{c}}(\mathbf{u}; \mathbf{o}, \mathbf{r}), \mathbf{0})) \\
&\quad - \lambda L(\mathbf{u}^*, \mathbf{o}; \mathbf{s}, \mathbf{r}) - \bar{J}(\mathbf{x}^*, \mathbf{z}^*; \mathbf{o}, \mathbf{r})) \\
&\quad - (\min_{\mathbf{u} \in \mathcal{U}} (\bar{J}(\mathbf{u}; \mathbf{o}, \mathbf{r}) - \beta^\top \min(\bar{\mathbf{c}}(\mathbf{u}; \mathbf{o}, \mathbf{r}), \mathbf{0})) - \bar{J}^*(\mathbf{o}; \mathbf{r})) \\
&\quad + (\lambda L(\mathbf{u}^*, \mathbf{o}; \mathbf{s}, \mathbf{r}) + \bar{J}(\mathbf{x}^*, \mathbf{z}^*; \mathbf{o}, \mathbf{r}) - \lambda L^*(\mathbf{o}; \mathbf{s}, \mathbf{r}) - \bar{J}^*(\mathbf{o}; \mathbf{r}))| \\
&\leq |\min_{\mathbf{u} \in \mathcal{U}} (\lambda L(\mathbf{u}, \mathbf{o}; \mathbf{s}, \mathbf{r}) + \bar{J}(\mathbf{u}; \mathbf{o}, \mathbf{r}) - \beta^\top \min(\bar{\mathbf{c}}(\mathbf{u}; \mathbf{o}, \mathbf{r}), \mathbf{0})) \\
&\quad - \lambda L(\mathbf{u}^*, \mathbf{o}; \mathbf{s}, \mathbf{r}) - \bar{J}(\mathbf{x}^*, \mathbf{z}^*; \mathbf{o}, \mathbf{r})| \\
&\quad + |\min_{\mathbf{u} \in \mathcal{U}} (\bar{J}(\mathbf{u}; \mathbf{o}, \mathbf{r}) - \beta^\top \min(\bar{\mathbf{c}}(\mathbf{u}; \mathbf{o}, \mathbf{r}), \mathbf{0})) - \bar{J}^*(\mathbf{o}; \mathbf{r})| \\
&\quad + |\lambda L(\mathbf{u}^*, \mathbf{o}; \mathbf{s}, \mathbf{r}) + \bar{J}(\mathbf{x}^*, \mathbf{z}^*; \mathbf{o}, \mathbf{r}) - \lambda L^*(\mathbf{o}; \mathbf{s}, \mathbf{r}) - \bar{J}^*(\mathbf{o}; \mathbf{r})| \\
&\quad < \frac{\lambda \epsilon_2}{3} + \frac{\lambda \epsilon_2}{3} + \frac{\lambda \epsilon_2}{3} = \lambda \epsilon_2
\end{aligned} \tag{50}$$

Note that  $\mathbf{u}^*$  is an optimal solution of (47) and  $\bar{J}^*(\mathbf{o}; \mathbf{r})$  is the optimal value of the original optimization stage (67). The first inequality is from the definition of the approximated loss function (45) and the triangle inequality. The second inequality is from the result of Step 1 and the definition of  $\delta_2, \delta_3$ . Therefore, the statement is proven.  $\square$

Therefore, we can use  $\tilde{L}(\mathbf{o}; \mathbf{s}, \mathbf{r}, \beta, \lambda)$  as our loss function for training since it is continuous with respect to the continuous part of  $\mathbf{o}$  and approach to  $L^*(\mathbf{o}; \mathbf{s}, \mathbf{r})$  when  $\lambda \rightarrow 0$  and  $\beta \rightarrow \infty$ .

## 5 Computation of gradient

In order to train the AI model, that is, to update parameters to minimize our approximate loss function, we need to obtain gradients of the approximated loss function with respect to the model parameters. The link between the AI model and the approximate loss function is the AI model output  $\mathbf{o} \in \mathcal{O} \subset R^{n_{oc}} \times N_0^{n_{od}}$  that has  $n_{oc}$  continuous elements and  $n_{od}$  discrete elements. Let  $\mathbf{o}_c \in \mathcal{O}_c \subset R^{n_{oc}}$  denotes the continuous part and  $\mathbf{o}_d \in \mathcal{O}_d \subset N_0^{n_{od}}$  denotes the discrete part. Since we cannot back-propagate gradients through the discrete part, we should deal with them in another way. We present the method to calculate the gradient for general output vector at first, and present specific way to calculate the gradient regarding the outputs from internal test cases.

## 5.1 General output

In this subsection, we deal with how to compute the gradient for general output vector (including discrete components). First, we present how to deal with the effect of infinitesimal change of parameters to the approximate loss function through the discrete part to train the AI model. We cannot directly define the gradient with respect to the discrete elements. However, these discrete elements are generally computed as a result of rounding or classification. For example, many classification models compute some real number associated with each class, and the class with the largest value can be regarded as the classification output. Thus, since continuous values are propagated between layers in AI models, discrete outputs can be considered as a sole function of some continuous interim results of the AI model.

We need to obtain the *virtual partial derivative* with respect to the continuous interim results to train the AI model. Although this is not the real gradient, this should be useful to update the model parameters to potentially result in a smaller approximate loss function. Let  $\mathbf{o}_d = (o_{d1}, o_{d2}, \dots, o_{dn_{od}}) \in \mathcal{O}_{d1} \times \mathcal{O}_{d2} \times \dots \mathcal{O}_{dn_{od}}$  and  $o_{di} = g_i(f(\mathbf{y}_i; \mathbf{w}_i)), f(\mathbf{y}_i; \mathbf{w}_i) \in \mathbb{R}^{m_i}, g_i: \mathbb{R}^{m_i} \rightarrow \mathcal{O}_{di}$ . Since  $g_i(f(\mathbf{y}_i; \mathbf{w}_i))$  is clearly discontinuous by definition and thus  $\tilde{L}(\mathbf{o}; \mathbf{s}, \mathbf{r}, \boldsymbol{\beta}, \lambda)$  is also discontinuous with respect to  $\mathbf{w}_i$ , we need to obtain the *softened approximated loss function* that is continuous and differentiable with respect to  $f(\mathbf{y}_i; \mathbf{w}_i)$ . Note that we assume that  $f(\mathbf{y}_i; \mathbf{w}_i)$  do not share elements with each other. If not, we can treat it as there are two copies of one variable, and then the effect of them will be added when we back-propagate the (approximate) gradient.

We construct the *softened approximated loss function* (51) for each  $f(\mathbf{y}_i; \mathbf{w}_i)$  as an expectation of  $\tilde{L}$  with respect to the stochastic selection of  $o_{di}$  via softened probability distribution  $p(o_{di}; f(\mathbf{y}_i; \mathbf{w}_i))$  for  $g_i(f(\mathbf{y}_i; \mathbf{w}_i))$ . The softened probability distribution  $p(o_{di}; f(\mathbf{y}_i; \mathbf{w}_i))$  can be set by various methods, but it needs to be continuous and partial-differentiable with respect to  $f(\mathbf{y}_i; \mathbf{w}_i)$  for any  $o_{di} \in \mathcal{O}_{di}$ . One example can be setting  $o_{di} = g_i(f(\mathbf{y}_i; \mathbf{w}_i) + \boldsymbol{\mu})$  for  $\boldsymbol{\mu}$  following standard normal distribution, i.e.,  $\mu_j \sim \mathcal{N}(0, 1) (j = 1, \dots, m_i)$ . Another example can be softmax. Note that  $\mathbf{o}_{d-i}$  denotes all elements of  $\mathbf{o}_d$  other than  $i$ th element.

$$EL_i(f(\mathbf{y}_i; \mathbf{w}_i); \mathbf{o}_c, \mathbf{o}_{d-i}, \mathbf{s}, \mathbf{r}, \boldsymbol{\beta}, \lambda) = \sum_{o_{di} \in \mathcal{O}_{di}} p(o_{di}; f(\mathbf{y}_i; \mathbf{w}_i)) \tilde{L}(\mathbf{o}_c, o_{di}, \mathbf{o}_{d-i}; \mathbf{s}, \mathbf{r}, \boldsymbol{\beta}, \lambda) \quad (51)$$

Then, since  $p(o_{di}; \mathbf{w}_i)$  is continuous and partial-differentiable with respect to  $f(\mathbf{y}_i; \mathbf{w}_i)$ , we can well-define *virtual partial derivative* with respect to  $f(\mathbf{y}_i; \mathbf{w}_i)$  as follows.

$$VPD_{di} := \frac{\partial}{\partial \mathbf{w}_i} EL_i(f(\mathbf{y}_i; \mathbf{w}_i); \mathbf{o}_c, \mathbf{o}_{d-i}, \mathbf{s}, \mathbf{r}, \boldsymbol{\beta}, \lambda) = \sum_{o_{di} \in \mathcal{O}_{di}} \frac{\partial p(o_{di}; f(\mathbf{y}_i; \mathbf{w}_i))}{\partial f(\mathbf{y}_i; \mathbf{w}_i)} \tilde{L}(\mathbf{o}_c, o_{di}, \mathbf{o}_{d-i}; \mathbf{s}, \mathbf{r}, \boldsymbol{\beta}, \lambda) \quad (52)$$

Gradient-descent method using this virtual partial derivative (52) decreases the probabil-



ity of high  $\tilde{L}$  and increases the probability of low  $\tilde{L}$  under noisy  $f(\mathbf{y}_i; \mathbf{w}_i)$ . This makes the AI model produce output  $\mathbf{o}$ , resulting in a low approximate loss function more frequently. Thus, we can use the virtual partial derivative (52) in AI model training as real gradients.

Now, we deal with the continuous elements. Theorem 2 guarantees only continuity, not differentiability of  $\tilde{L}(\mathbf{o}; \mathbf{s}, \mathbf{r}, \boldsymbol{\beta}, \lambda)$ . Thus, we need to obtain the *virtual partial derivative* of  $\tilde{L}$ , which can be used as real gradients for training when it is not differentiable. Similar to the definition of gradient, we can define our *virtual partial derivative* as equation (53). Note that  $\mathbf{o}_{c-i}$  denotes all elements of  $\mathbf{o}_c$  other than  $i$ th element, and we can arbitrarily choose sufficiently small  $\rho$ .

$$VPD_{ci} := \frac{1}{\rho o_{ci}} (\tilde{L}((o_{ci} + \rho o_{ci}, \mathbf{o}_{c-i}, \mathbf{o}_d); \mathbf{s}, \mathbf{r}, \boldsymbol{\beta}, \lambda) - \tilde{L}(\mathbf{o}; \mathbf{s}, \mathbf{r}, \boldsymbol{\beta}, \lambda)) \quad (53)$$

In some cases, we can obtain the exact gradient by differentiating  $\tilde{L}(\mathbf{o}; \mathbf{s}, \mathbf{r}, \boldsymbol{\beta}, \lambda)$ . For simplicity, we let  $P(\mathbf{u}, \mathbf{o}; \mathbf{s}, \mathbf{r}) := \lambda L(\mathbf{u}, \mathbf{o}; \mathbf{s}, \mathbf{r}) + \bar{J}(\mathbf{u}; \mathbf{o}, \mathbf{r}) - \boldsymbol{\beta}^\top \min(\bar{\mathbf{c}}(\mathbf{u}; \mathbf{o}, \mathbf{r}), \mathbf{0})$  and  $Q(\mathbf{u}, \mathbf{o}; \mathbf{r}) := \bar{J}(\mathbf{u}; \mathbf{o}, \mathbf{r}) - \boldsymbol{\beta}^\top \min(\bar{\mathbf{c}}(\mathbf{u}; \mathbf{o}, \mathbf{r}), \mathbf{0})$ . Then, a set of conditions sufficient for the analytical calculation of the gradient is presented in Condition 4.

**Condition 4.** For given  $\mathbf{s}, \mathbf{r}$ , and  $\mathbf{o}_0$ , there exists  $\epsilon_4(\mathbf{s}, \mathbf{r}, \mathbf{o}_0) > 0$  that makes the following statements satisfy in neighborhood  $B(\mathbf{o}_{c0}, \epsilon_4) \times \{\mathbf{o}_{d0}\} \subset \mathcal{O}$ .

1.  $P(\mathbf{u}, \mathbf{o}; \mathbf{s}, \mathbf{r})$  and  $Q(\mathbf{u}, \mathbf{o}; \mathbf{r})$  have gradients with respect to  $\mathbf{o}_c$  at  $\mathbf{o}_c = \mathbf{o}_{c0}$ .
2.  $P(\mathbf{u}, \mathbf{o}; \mathbf{s}, \mathbf{r})$  and  $Q(\mathbf{u}, \mathbf{o}; \mathbf{r})$  have only one minimum  $(\mathbf{x}_p(\mathbf{o}), \mathbf{z}_p(\mathbf{o})) \in \mathcal{U}$ ,  $(\mathbf{x}_q(\mathbf{o}), \mathbf{z}_q(\mathbf{o})) \in \mathcal{U}$ , respectively.

That is,  $\{(\mathbf{x}_p, \mathbf{z}_p)\} = \arg \min_{\mathbf{u} \in \mathcal{U}} (\lambda L(\mathbf{u}, \mathbf{o}; \mathbf{s}, \mathbf{r}) + \bar{J}(\mathbf{u}; \mathbf{o}, \mathbf{r}) - \boldsymbol{\beta}^\top \min(\bar{\mathbf{c}}(\mathbf{u}; \mathbf{o}, \mathbf{r}), \mathbf{0}))$ ,  $\{(\mathbf{x}_q, \mathbf{z}_q)\} = \arg \min_{\mathbf{u} \in \mathcal{U}} (\bar{J}(\mathbf{u}; \mathbf{o}, \mathbf{r}) - \boldsymbol{\beta}^\top \min(\bar{\mathbf{c}}(\mathbf{u}; \mathbf{o}, \mathbf{r}), \mathbf{0}))$

3.  $\mathbf{x}_p(\mathbf{o})$  and  $\mathbf{x}_q(\mathbf{o})$  have gradients with respect to  $\mathbf{o}_c$  at  $\mathbf{o}_0$ .
4.  $\mathbf{z}_p(\mathbf{o})$  and  $\mathbf{z}_q(\mathbf{o})$  are constant.
5.  $(\mathbf{x}_p(\mathbf{o}_0), \mathbf{z}_p(\mathbf{o}_0))$  and  $(\mathbf{x}_q(\mathbf{o}_0), \mathbf{z}_q(\mathbf{o}_0))$  are in the interior of  $\mathcal{U}$ .

Then, we derive the exact gradient of  $\tilde{L}(\mathbf{o}; \mathbf{s}, \mathbf{r}, \boldsymbol{\beta}, \lambda)$  with respect to  $\mathbf{o}$  under Condition 4 in Theorem 6.

**Proposition 6.** Under Assumption 1, Assumption 2, and Condition 4, gradient of  $\tilde{L}(\mathbf{o}; \mathbf{s}, \mathbf{r}, \boldsymbol{\beta}, \lambda)$  with respect to  $\mathbf{o}_c$  at  $\mathbf{o}_0$  can be calculated as follows.

$$\nabla_{\mathbf{o}_c} \tilde{L}(\mathbf{o}; \mathbf{s}, \mathbf{r}, \boldsymbol{\beta}, \lambda)(\mathbf{o}_0) = \frac{1}{\lambda} (\nabla_{\mathbf{o}_c} P(\mathbf{x}_p, \mathbf{o}_0) - \nabla_{\mathbf{o}_c} Q(\mathbf{x}_q, \mathbf{o}_0)) \quad (54)$$

*Proof.* Under Assumption, 1, Assumption 2, and Condition 4, equation (55) is a direct result of the chain rule. Note that the effect of the gradient of  $\mathbf{z}$  with respect to  $\mathbf{o}$  is 0

because of statement 4 of Condition 4.

$$\begin{aligned} \nabla_{\mathbf{o}_c} \tilde{L}(\mathbf{o}; \mathbf{s}, \mathbf{r}, \beta, \lambda)(\mathbf{o}_0) = & \frac{1}{\lambda} (\nabla_{\mathbf{o}_c} P(\mathbf{x}_p, \mathbf{o}_0) + \nabla_{\mathbf{x}} P(\mathbf{x}_p, \mathbf{o}_0) \nabla_{\mathbf{o}_c} \mathbf{x}_p(\mathbf{o}_0) \\ & - \nabla_{\mathbf{o}_c} Q(\mathbf{x}_q, \mathbf{o}_0) - \nabla_{\mathbf{x}} Q(\mathbf{x}_q, \mathbf{o}_0) \nabla_{\mathbf{o}_c} \mathbf{x}_q(\mathbf{o}_0)) \end{aligned} \quad (55)$$

Then, by the fifth statement of Condition 4, constraints  $\mathbf{u} \in \mathcal{U}$  do not affect  $\nabla_{\mathbf{o}_c} \mathbf{x}_p(\mathbf{o}_0)$  and  $\nabla_{\mathbf{o}_c} \mathbf{x}_q(\mathbf{o}_0)$ . Thus, as a sole minimality condition, we need to consider only stationarity with respect to  $\mathbf{x}$ , that is,

$$\nabla_{\mathbf{x}} P(\mathbf{x}_p, \mathbf{o}_0) = \nabla_{\mathbf{x}} Q(\mathbf{x}_q, \mathbf{o}_0) = 0 \quad (56)$$

Therefore, (55) reduces to (54).  $\square$

Note that Condition 4 generally holds for problems we usually solve. The reason can be stated as follows. Most of the basic functions we deal with (polynomial, exponential, trigonometric, etc.) are differentiable, and thus statement 1 and statement 3 hold. Other statements are similar to nonsingularity conditions that hold almost everywhere. The key point of Theorem 6 is the elimination of gradients with respect to  $\mathbf{x}$ , and this is the direct result of minimization in the definition of  $\tilde{L}$ . Since we can choose arbitrarily big  $\mathcal{U}$  as long as it is bounded and functions are well-defined in which, we can easily satisfy the fifth condition that removes the effect of constraints.

As the final part of this subsection, we summarize the computational cost of calculating (virtual) gradient in units of computational cost solving minimization problem in Theorem 7. This is important since we do not constrain the type of our optimization problem, and thus, the minimization can take much longer time than other operations.

**Proposition 7.** *When all  $\mathcal{O}_{di}(1 \leq i \leq n_{od})$  are finite, the number of times we need to solve minimization problems (of  $P$  or  $Q$ ) to obtain virtual or exact gradients with respect to all elements of AI model output is as follows.*

1. *When we use equation (53) to obtain virtual gradients with respect to continuous elements:  $2 \times (2n_{oc} + \sum_i^{n_{od}} |\mathcal{O}_{di}|)$*
2. *When we use equation (54) to obtain exact gradients with respect to continuous elements and  $\nabla_{\mathbf{o}_c} P$  and  $\nabla_{\mathbf{o}_c} Q$  are (locally) known analytically:  $2 \times (1 + \sum_i^{n_{od}} |\mathcal{O}_{di}|)$*

*Proof.* By definition of virtual partial derivative with respect to a discrete element (52), calculating it needs computation of  $\tilde{L}$  for all  $\mathbf{o}_{di}$ . Thus, the calculation of the virtual partial derivative with respect to all discrete elements requires  $2 \times \sum_i^{n_{od}} |\mathcal{O}_{di}|$  times of minimization since one computation of  $\tilde{L}$  needs two minimizations.

Meanwhile, (53) needs two times of computation of  $\tilde{L}$  for each continuous element of  $\mathbf{o}$ , which means 4 times of minimization are needed. As a result,  $2 \times (2n_{oc} + \sum_i^{n_{od}} |\mathcal{O}_{di}|)$

times of minimization are needed to find (virtual) gradient for whole output when we use equation (53).

In contrast, computation of (54) requires only two times of minimization when we already know the analytical expression of  $\nabla_{\mathbf{o}_c} P$  and  $\nabla_{\mathbf{o}_c} Q$  locally. This provides partial derivatives for all continuous elements of  $\mathbf{o}$  simultaneously. Therefore, we need only  $2 \times (1 + \sum_i^{n_{od}} |\mathcal{O}_{di}|)$  times of minimization.  $\square$

## 5.2 Gradients for internal test cases

In this subsection, we present the techniques for the computation of the (approximate) gradient of the approximate loss function with the conservative testing technique for the training of the chance-constrained method in the framework. For simplicity, we define  $\mathbf{N}^\xi$  as  $(N^{+\xi}, N^{-\xi})$ . By starting from the definition (52), we can calculate the virtual partial gradient for the chance-constrained part (with conservative testing technique) as

$$VPD_{cr}^\xi = \sum_k^{n_t} \sum_{\{\mathbf{N}_{\mathbf{s}_{cr}=\bar{\mathbf{s}}_i, \mathbf{o}_{cr}=\bar{\mathbf{o}}_j}^\xi\}} \frac{\partial Pr^\xi(\{\mathbf{N}_{\mathbf{s}_{cr}=\bar{\mathbf{s}}_i, \mathbf{o}_{cr}=\bar{\mathbf{o}}_j}^\xi\})}{\partial f(\mathbf{y}_{cr}^{t_k}; \mathbf{w}_{cr})} \tilde{L}(\{\mathbf{N}_{\mathbf{s}_{cr}=\bar{\mathbf{s}}_i, \mathbf{o}_{cr}=\bar{\mathbf{o}}_j}^\xi\}, \mathbf{o}_{ncr}; \mathbf{s}, \mathbf{r}, \boldsymbol{\beta}, \lambda) \quad (57)$$

when  $Pr^\xi(\{\mathbf{N}_{\mathbf{s}_{cr}=\bar{\mathbf{s}}_i, \mathbf{o}_{cr}=\bar{\mathbf{o}}_j}^\xi\})$  is defined as the probability of  $\{\mathbf{N}_{\mathbf{s}_{cr}=\bar{\mathbf{s}}_i, \mathbf{o}_{cr}=\bar{\mathbf{o}}_j}^\xi\}$  under  $p^{+\xi}(\bar{\mathbf{o}}_j; f(\mathbf{y}_{cr}^{t_k}, \mathbf{w}_{cr}))$ : smoothed version of  $\mathbf{1}^{+\xi}(\mathbf{o}_{cr}^{t_k}, \bar{\mathbf{o}}_j)$  (same with  $-\xi$ ).

Then, by using the chain rule and defining  $\{\mathbf{N}_{\mathbf{s}_{cr}=\bar{\mathbf{s}}_i, \mathbf{o}_{cr}=\bar{\mathbf{o}}_j}^{\xi, -k}\}$  as the number of (internal) test cases for each environment state and output without  $k$  th test case, we can convert it as

$$\begin{aligned} VPD_{cr}^\xi &= \sum_k^{n_t} \sum_{\{\mathbf{N}_{\mathbf{s}_{cr}=\bar{\mathbf{s}}_i, \mathbf{o}_{cr}=\bar{\mathbf{o}}_j}^\xi\}} \frac{\partial Pr^\xi(\{\mathbf{N}_{\mathbf{s}_{cr}=\bar{\mathbf{s}}_i, \mathbf{o}_{cr}=\bar{\mathbf{o}}_j}^\xi\})}{\partial f(\mathbf{y}_{cr}^{t_k}; \mathbf{w}_{cr})} E(\tilde{L}; \{\mathbf{N}_{\mathbf{s}_{cr}=\bar{\mathbf{s}}_i, \mathbf{o}_{cr}=\bar{\mathbf{o}}_j}^\xi\}) \\ &= \sum_k^{n_t} \left( \sum_{\{\mathbf{N}_{\mathbf{s}_{cr}=\bar{\mathbf{s}}_i, \mathbf{o}_{cr}=\bar{\mathbf{o}}_j}^{\xi, -k}\}} \sum_l \frac{\partial p^{+\xi}(\bar{\mathbf{o}}_l; f(\mathbf{y}_{cr}^{t_k}, \mathbf{w}_{cr}))}{\partial f(\mathbf{y}_{cr}^{t_k}; \mathbf{w}_{cr})} Pr^\xi(\{\mathbf{N}_{\mathbf{s}_{cr}=\bar{\mathbf{s}}_i, \mathbf{o}_{cr}=\bar{\mathbf{o}}_j}^{\xi, -k}\}) \right. \\ &\quad (E(\tilde{L}; \{\mathbf{N}_{\mathbf{s}_{cr}=\bar{\mathbf{s}}_i, \mathbf{o}_{cr}=\bar{\mathbf{o}}_1}^{\xi, -k}, \dots, \mathbf{N}_{\mathbf{s}_{cr}=\bar{\mathbf{s}}_i, \mathbf{o}_{cr}=\bar{\mathbf{o}}_{l-1}}^{\xi, -k}, \mathbf{N}_{\mathbf{s}_{cr}=\bar{\mathbf{s}}_i, \mathbf{o}_{cr}=\bar{\mathbf{o}}_l}^{\xi, -k} + (1, 0), \\ &\quad \mathbf{N}_{\mathbf{s}_{cr}=\bar{\mathbf{s}}_i, \mathbf{o}_{cr}=\bar{\mathbf{o}}_{l+1}}^{\xi, -k}, \dots, \mathbf{N}_{\mathbf{s}_{cr}=\bar{\mathbf{s}}_i, \mathbf{o}_{cr}=\bar{\mathbf{o}}_{N_o}}^{\xi, -k}\}) - E(\tilde{L}; \{\mathbf{N}_{\mathbf{s}_{cr}=\bar{\mathbf{s}}_i, \mathbf{o}_{cr}=\bar{\mathbf{o}}_j}^{\xi, -k}\})) \\ &\quad + \sum_{\{\mathbf{N}_{\mathbf{s}_{cr}=\bar{\mathbf{s}}_i, \mathbf{o}_{cr}=\bar{\mathbf{o}}_j}^{\xi, -k}\}} \sum_l \frac{\partial p^{-\xi}(\bar{\mathbf{o}}_l; f(\mathbf{y}_{cr}^{t_k}, \mathbf{w}_{cr}))}{\partial f(\mathbf{y}_{cr}^{t_k}; \mathbf{w}_{cr})} Pr^\xi(\{\mathbf{N}_{\mathbf{s}_{cr}=\bar{\mathbf{s}}_i, \mathbf{o}_{cr}=\bar{\mathbf{o}}_j}^{\xi, -k}\}) \\ &\quad (E(\tilde{L}; \{\mathbf{N}_{\mathbf{s}_{cr}=\bar{\mathbf{s}}_i, \mathbf{o}_{cr}=\bar{\mathbf{o}}_1}^{\xi, -k}, \dots, \mathbf{N}_{\mathbf{s}_{cr}=\bar{\mathbf{s}}_i, \mathbf{o}_{cr}=\bar{\mathbf{o}}_{l-1}}^{\xi, -k}, \mathbf{N}_{\mathbf{s}_{cr}=\bar{\mathbf{s}}_i, \mathbf{o}_{cr}=\bar{\mathbf{o}}_l}^{\xi, -k} + (0, 1), \\ &\quad \mathbf{N}_{\mathbf{s}_{cr}=\bar{\mathbf{s}}_i, \mathbf{o}_{cr}=\bar{\mathbf{o}}_{l+1}}^{\xi, -k}, \dots, \mathbf{N}_{\mathbf{s}_{cr}=\bar{\mathbf{s}}_i, \mathbf{o}_{cr}=\bar{\mathbf{o}}_{N_o}}^{\xi, -k}\}) - E(\tilde{L}; \{\mathbf{N}_{\mathbf{s}_{cr}=\bar{\mathbf{s}}_i, \mathbf{o}_{cr}=\bar{\mathbf{o}}_j}^{\xi, -k}\})) \end{aligned} \quad (58)$$

when  $E(\tilde{L}; \{\mathbf{N}_{\mathbf{s}_{cr}=\mathbf{s}_{cr}^{t_k}, \mathbf{o}_{cr}=\bar{\mathbf{o}}_j}^\xi\})$  is the expectation of  $\tilde{L}$  under  $\{\mathbf{N}_{\mathbf{s}_{cr}=\mathbf{s}_{cr}^{t_k}, \mathbf{o}_{cr}=\bar{\mathbf{o}}_j}^\xi\}$  (with probabilistic  $\{\mathbf{N}_{\mathbf{s}_{cr}=\bar{\mathbf{s}}_i, \mathbf{o}_{cr}=\bar{\mathbf{o}}_j}^\xi\}$  for  $\bar{\mathbf{s}}_i \neq \mathbf{s}_{cr}^{t_k}$ )

As an alternative way, we can make a continuous approximate function of  $\tilde{L}$  for continuous  $\tilde{N}_{\mathbf{s}_{cr}=\bar{\mathbf{s}}_i, \mathbf{o}_{cr}=\bar{\mathbf{o}}_j}^{+\xi} := \sum_{k=1}^{n_t} \mathbf{1}(\mathbf{s}_{cr}^{t_k}, \bar{\mathbf{s}}_i) p^{+\xi}(\bar{\mathbf{o}}_l; f(\mathbf{y}_{cr}^{t_k}; \mathbf{w}_{cr}))$  and  $\tilde{N}_{\mathbf{s}_{cr}=\bar{\mathbf{s}}_i, \mathbf{o}_{cr}=\bar{\mathbf{o}}_j}^{-\xi} := \sum_{k=1}^{n_t} \mathbf{1}(\mathbf{s}_{cr}^{t_k}, \bar{\mathbf{s}}_i) p^{-\xi}(\bar{\mathbf{o}}_l; f(\mathbf{y}_{cr}^{t_k}; \mathbf{w}_{cr}))$ . More details about the technique are provided with empirical examples.

## 6 Scaling Law

To mathematically deal with the scaling law, we review the concept of  $\zeta$ -coverage introduced in [accepted previous paper].

**Definition 3.** [Slightly modified from Definition 1 in [accepted previous paper]] For  $\zeta > 0$ , we call a dataset  $D$  is  $\zeta$ -coverage if and only if  $D$  satisfies the following:

$$\cup_{\omega \in D} B(\omega, \zeta) = \Omega, \quad (59)$$

where  $B(\omega, \zeta)$  is an open ball with radius  $\zeta$  centered at  $\omega$ .

Now, we construct the safe set based on the internal test data with this concept. Our main method to identify the safe set well is as follows: We employ internal test data in the product of the input space and the action space (denote as  $\Omega^*$ ). Then, we consider a radius  $\zeta$  that make the internal test data be  $\zeta$ -coverage [accepted previous paper], which is the condition that the union of  $\zeta$ -balls centered on the data contains the whole product space. Next, when we classify all data within  $\zeta$ -range from a internal test data which is safe, our safe set classification can be a estimate of the real safe set. The probability of first and second type error (misclassification of unsafe action as safe and vise versa) is upper-bounded with the difference of the probability of real safe set and  $\zeta$ -inflated real safe set and the difference of the probability of real unsafe set and  $\zeta$ -inflated real unsafe set.

When we use more internal test data, we can use smaller  $\zeta$  and thus the probability of set difference becomes smaller. Conversely, when we decide the probability bound, we can decide the appropriate  $\zeta$  to ensure it (with some condition of the real safe set). Then, we can compute the expectation of required number of internal test data to ensure  $\zeta$ -coverage with such  $\zeta$ . With the process, under the following conditions, we can obtain the following theorem.

**Condition 5.** 1.  $\Omega^*$  is a compact metric space with endowed probability measure  $P^*$  that is defined on a Borel  $\sigma$ -algebra.

2. There exists a well-defined safe set  $S$  that includes all pairs of input and action satisfy the constraint. That is, the safe and unsafe pairs of input and action can be completely distinguishable in principle.

3. the safe set  $S$  and its complement  $\Omega^* \setminus S$  have finite boundary probability measure for dimension  $d - 1$ , that is,

$$\limsup_{r \rightarrow 0^+} \frac{P^*(\cup_{\Omega^* \in S} B(\Omega^*, \zeta) \setminus S)}{r}, \limsup_{r \rightarrow 0^+} \frac{P^*(\cup_{\Omega^* \in \Omega^* \setminus S} B(\Omega^*, \zeta) \setminus (\Omega^* \setminus S))}{r} < \infty \quad (60)$$

**Condition 6.** All open balls with radius  $r$  in the input space  $\Omega^*$  have probability measure of at least  $r^d$  with constant  $\kappa r^d$ .

**Theorem 3.** Under condition 5 and 6, when we assume that we can define safety classification model as an arbitrary partition of  $\Omega^*$ , the expected number  $N_{reqit}$  of required internal test data to upper-bound both the first type error and second-type error probability as  $p$  grows as

$$N_{reqit} \leq Ap^{-d} \quad (61)$$

when  $A$  is the constant and  $d$  is the dimension of the input space.

*Proof.* For simplicity, let  $t_1, \dots, t_{N_{sit}} (\in S)$  as safe internal test data and  $t_{N_{sit}+1}, \dots, t_{N_{sit}+N_{usit}} (\in \Omega^* \setminus S)$  ( $N_{sit} + N_{usit} = n_t$ ) as unsafe internal test data. For  $\zeta$  that makes the internal test data  $t_1, \dots, t_{n_t}$  be  $\zeta$ -coverage of  $\Omega^*$ , we classify pairs of input and action in  $\cup_{i=1}^{n_{sit}} B(t_i, \zeta)$  as safe.

Part 1. Computation appropriate  $\zeta$  to upper bound the error probabilities

In this part, we compute the required  $\zeta$  to upper bound the error probabilities to  $p$ . Then, the first and second type error probabilities are

$$\frac{P^*(S \setminus \cup_{i=1}^{n_{sit}} B(t_i, \zeta))}{P^*(S)}, \frac{P^*(\cup_{i=1}^{n_{sit}} B(t_i, \zeta) \setminus S)}{P^*(\Omega^* \setminus S)}, \quad (62)$$

respectively. Based on the  $\zeta$ -coverage assumption, we have

$$\frac{P^*(S \setminus \cup_{i=1}^{n_{sit}} B(t_i, \zeta))}{P^*(S)} \leq \frac{P^*(S \setminus (\Omega^* \setminus (\cup_{i=N_{sit}+1}^{N_{sit}+N_{usit}} B(t_i, \zeta))))}{P^*(S)} = \frac{P^*(S \cap (\cup_{i=N_{sit}+1}^{N_{sit}+N_{usit}} B(t_i, \zeta)))}{P^*(S)} \quad (63)$$

Since unsafe internal test data is not included in the safe set, we can obtain

$$\frac{P^*(S \cap (\cup_{i=N_{sit}+1}^{N_{sit}+N_{usit}} B(t_i, \zeta)))}{P^*(S)} \leq \frac{P^*(S \cap (\cup_{\Omega^* \in \Omega^* \setminus S} B(\Omega^*, \zeta)))}{P^*(S)} = \frac{P^*((\cup_{\Omega^* \in \Omega^* \setminus S} B(\Omega^*, \zeta) \setminus (\Omega^* \setminus S)))}{P^*(S)} \quad (64)$$

Conversely, since all safe internal test data is included in  $S$ , we can obtain

$$\frac{P^*(\cup_{i=1}^{n_{sit}} B(t_i, \zeta) \setminus S)}{P^*(\Omega^* \setminus S)} \leq \frac{P^*(\cup_{\Omega^* \in S} B(\Omega^*, \zeta) \setminus S)}{P^*(\Omega^* \setminus S)} \quad (65)$$

By condition 5, we have  $(k_s, r_s)$  and  $(k_{us}, r_{us})$  that satisfy  $\forall r < r_s, P^*(\cup_{\Omega^* \in S} B(\Omega^*, \zeta) \setminus$

$S) < k_s r_s$  and  $\forall r < r_{us}, P^*(\cup_{\Omega^* \in \Omega^* \setminus S} B(\Omega^*, \zeta) \setminus (\Omega^* \setminus S)) < k_{us} r_{us}$ , respectively. Now, when  $\zeta$  satisfies  $\zeta \leq \min(r_s, r_{us}, \frac{pP^*(S)}{k_{us}}, \frac{pP^*(\Omega^* \setminus S)}{k_s})$ , both the first and the second type error probabilities are lower than or equal to  $p$ .

Part 2. Computation of expected number of required internal test data to be  $\zeta$ -coverage with such  $\zeta$ .

In this part, we compute how many internal test data are needed to be  $\zeta$ -coverage with  $\zeta := \min(r_s, r_{us}, \frac{pP^*(S)}{k_{us}}, \frac{pP^*(\Omega^* \setminus S)}{k_s})$ . Since  $\Omega^*$  is compact, we can obtain a finite subcover of open cover  $\{B(\Omega^*, \frac{\zeta}{2}) | \Omega^* \in \Omega^*\}$ . Based on condition 6 the open balls consisting of the finite subcover have probability measure of at least  $\frac{\kappa \zeta^d}{2^d}$ .

Then, when we sample  $n_t$  internal test data, all open balls in the subcover have at least one sampled element with probability at least  $1 - (1 - \frac{\kappa \zeta^d}{2^d})^{n_t}$ . Letting the size of the finite subcover as  $N_{sc}$ , By union bound, for probability at least  $1 - N_{sc}(1 - \frac{\kappa \zeta^d}{2^d})^{n_t}$ , all open balls in the subcover have at least one internal test data. Considering the radius of the open ball is  $\frac{\zeta}{2}$ , this means all elements in the subcover is subset of  $\cup_{i=1}^{n_t} B(t_i, \zeta)$ , and thus, this internal test data are  $\zeta$ -coverage.

Now, we can compute the expected number of the internal test data to be  $\zeta$ -coverage as follows (with a constant  $A$ ).

$$\begin{aligned} N_{reqit} &\leq \sum_{n_t} n_t Pr_{n_t}(\{t_1, \dots, t_{n_t}\}: \zeta\text{-coverage}, \{t_1, \dots, t_{N_t-1}\}: \text{not } \zeta\text{-coverage}) \\ &= \sum_{n_t} Pr_{n_t}(\{t_1, \dots, t_{n_t}\}: \text{not } \zeta\text{-coverage}) = \sum_{n_t} (1 - \frac{\kappa \zeta^d}{2^d})^{n_t} = \frac{2^d}{\kappa \zeta^d} \quad (66) \\ &= \frac{2^d}{\kappa \min(r_s, r_{us}, \frac{pP^*(S)}{k_{us}})^d} \leq Ap^{-d} \end{aligned}$$

□

## 7 Bias Correction to Tailor to User-Given Threshold in Utilization

In the utilization stage, the computed posterior of outputs  $p^\xi(\mathbf{s}_{cr} = \bar{\mathbf{s}}_i | \mathbf{o}_{cr} = \bar{\mathbf{o}}_j)$  are discrete since the number of possible constraint-related environment states and outputs are finite by assumption. If we fix the model, the system based on our framework can only tackle user-given threshold as step-like manner. For instance, if the threshold is lower than  $\min_{i,j} p^\xi(\mathbf{s}_{cr} = \bar{\mathbf{s}}_i | \mathbf{o}_{cr} = \bar{\mathbf{o}}_j)$ , we should satisfy all constraints included in chance-constraints. This is inefficient since we cannot smoothly adjust the system regarding the user-given threshold.

Alternatively, in the utilization stage, we modify our AI model by adding a constant

vector to the final layer output,  $f'(\mathbf{y}; \mathbf{w}_{cr}) = f(\mathbf{y}; \mathbf{w}_{cr}) + \mathbf{v}$ , which is equivalent to adding  $\mathbf{v}$  to the final layer bias. Then, we can treat  $f'(\mathbf{y}; \mathbf{w}_{cr})$  as the final layer output of new AI model and obtain new output  $\mathbf{o}'_{cr}$ . Note that  $\mathbf{v}$  can be any constant vector that have same dimension with  $f(\mathbf{y}; \mathbf{w}_{cr})$ . Whole theory discussed so far still holds for  $f'(\mathbf{y}; \mathbf{w}_{cr})$  and  $\mathbf{o}'_{cr}$ . Thus, we may adjust the AI model output to obtain better performance.

In the beginning of the utilization stage, we can run inference for the internal test data first. Then, we can find  $\mathbf{v}$  that makes the computed posterior  $p^\xi(\mathbf{s}_{cr} = \bar{\mathbf{s}}_i | \mathbf{o}'_{cr} = \bar{\mathbf{o}}_j)$  or to be desired values. For instance, when there are only two environment states and two outputs class, we can set  $\mathbf{v}$  that makes  $p^\xi(\mathbf{s}_{cr} = \bar{\mathbf{s}}_1 | \mathbf{o}'_{cr} = \bar{\mathbf{o}}_1)$  or  $p^\xi(\mathbf{s}_{cr} = \bar{\mathbf{s}}_1 | \mathbf{o}'_{cr} = \bar{\mathbf{o}}_2)$  be same with threshold  $r_t$  (if such  $\mathbf{v}$  exists) to avoid constraint associated to  $\bar{\mathbf{s}}_1$  as much as possible through  $\bar{\mathbf{o}}_1$  or  $\bar{\mathbf{o}}_2$ , respectively. (Same thing holds for  $\bar{\mathbf{s}}_2$ .) Implementation details are provided in part 2 of the supplementary material.

## 8 Constrained Action Sampling

In this section, we introduce a special but widely applicable approach of the proposed framework, constrained action sampling. When we want to ensure safety with an AI model that generates action candidates (e.g. generative AI or RL applications), we can use this framework to choose a safe action among the candidates. We present full characterization below.

Suppose we deal with  $n$  action candidates generated by an AI model. At first, we define the environment state as a  $n$ -dimensional binary vector,  $\mathbf{s} = \mathbf{s}_{cr} = (s_1, \dots, s_n)$  (whole components of  $\mathbf{s}$  is constraint-related), with  $s_k$  is 1 if  $k$ th action candidate is unsafe and 0 if safe. We define the output as  $2n$ -dimensional vector, that includes weights of action candidates generated by action generating model generates as  $o_{w1}, \dots, o_{wn}$  and safety classification results for the action candidates  $o_{c1}, \dots, o_{cn}$ . Note that  $\mathbf{o} = (o_{w1}, \dots, o_{wn}, o_{c1}, \dots, o_{cn})$  and  $\mathbf{o}_{cr} = (o_{c1}, \dots, o_{cn})$  since weights are not directly related to safety.

Now, we can construct the optimization problem as follows:

$$\min_{z \sim [o_{w1}, \dots, o_{wn}] \forall z = \hat{d}} \bar{J}(z) \quad (67a)$$

$$\text{subject to} \quad z \neq i \vee p^\xi(s_i = 1 | o_i) \leq r_t, \quad i = 1, \dots, n \quad (67b)$$

When  $\hat{d}$  denotes default action, which is set to be used only when all actions have larger constraint-violation posterior than threshold  $r_t$  ( $\forall i, p^\xi(s_i = 1 | o_i) > r_t$ ), by setting  $\bar{J}(\hat{d}) > 0 = \bar{J}(1) = \dots = \bar{J}(n)$ . Note that  $z \sim [o_{w1}, \dots, o_{wn}]$  means  $z$  follows the probability distribution defined by the weights  $o_{w1}, \dots, o_{wn}$ .<sup>1</sup>

---

<sup>1</sup>This kind of sampling can be easily converted to traditional optimization problem by introducing a random variable added to  $\bar{J}(i)$  following the probability distribution.

Although we state the case that action candidates are generated by an AI model, we can easily apply same approach when action candidates are fixed and only distribution (weights) are provided by the AI model. We also extend this approach by combining with traditional optimization problem to apply the case that some part of action should be sampled and the other part should be optimized traditionally. With this approach, the internal test cases should be safety-labeled action candidates (concatenated with the problem or given information for action generation and considering safety) generated by same AI model. Then, the distribution of the actions obtained by this approach is exactly same with the distribution of action samples with safety classification model output satisfying  $p^\xi(s_i = 1|o_i) \leq r_t$  because both apply same condition (for the safety classification model output) onto same distribution (generated by same AI model), thus, this approach ensure safety.

## 9 Application to RL

Reinforcement learning (RL) algorithms allow us to deal with problems where the rewards are given as a function of a sequence of outputs rather than one output. In this section, we provide a combination of our proposed system and an RL algorithm to deal with such problems with guaranteeing safety. In most of RL applications, the agent can get into unsafe situation as a result of a series of action and some potential external intervention or noise. We should deal with this as a nondeterministic constraint and carefully define the constraint violation. Since we cannot determine the constraint satisfaction for an infinite number of actions, we employ a constrained action sampling approach by employing an existing RL algorithm that provides action samples or their distribution. We let the loss for the action samples as 0 to ensure random sampling without preference.

Conversely, from the point of view of reinforcement learning, our system is a policy. The policy provided by reinforcement learning algorithm is now just a distribution (or action sample) generating component of our system, which act as the policy as a whole. Optimization problem can be considered as policy refining stage.

In this paper, even though we expect that our system can be combined with a variety of RL algorithms by replacing their policy part, we present how our system can be combined with policy optimization based algorithms such as proximal policy optimization (PPO) and trust region policy optimization (TRPO). The policy component of the algorithm samples the action from a normal distribution characterized by mean and standard deviation. We discretize the action space into fixed action samples. Then, we compute the weight of each action sample based on the probability density function of the normal distribution. Finally, we sample our action through constrained action sampling. The detailed algorithm is presented in experiment part with the internal test data collection.



## 9.1 Internal test data collection

Intrinsically, internal test data are samples of the potential situations that our system encounters in the problem. We define the safety label as whether the action lead to unsafe situation within the predefined length of time steps. Then, internal test data are state and action records with safety labels. Considering this point, internal test data can be sampled through internal test data collection process, which is execution of the RL algorithm within the simulator and saving the states and actions with the safety label, prior to the training of the whole system. Unfortunately, obviously, safety cannot be guaranteed in these executions. Note that guaranteeing safety without any information about safety is fundamentally impossible.

In addition to the internal test data collection process, internal test data can be added or updated in accordance with the instructions given by the user. For the detailed algorithm, please refer to the experiment part.
